# Supplementary material for: Inverse Design of Ultralow Lattice Thermal Conductivity Materials Via Lone Pair Cation Coordination Environment
Source: arXiv:2004.01579 source file (2020-04-03)
Supplement: Supplementary file 1 [file si_smaller.pdf]

# Supporting Information for "Inverse Design of Ultralow Lattice Thermal Conductivity Materials Via Lone Pair Cation Coordination Environment"

Eric B. Isaacs,[†] Grace M. Lu,[†,‡] and Christopher Wolverton[*,†]

†*Department of Materials Science and Engineering, Northwestern University, Evanston, Illinois 60208, USA*

‡*Present Address: Department of Materials Science and Engineering, University of Illinois at Urbana-Champaign, Urbana, IL 61801, USA*

E-mail: c-wolverton@northwestern.edu

## Characterization of 352 compounds passing initial screening criteria

Here, we characterize the 352 compounds passing the initial screening criteria.

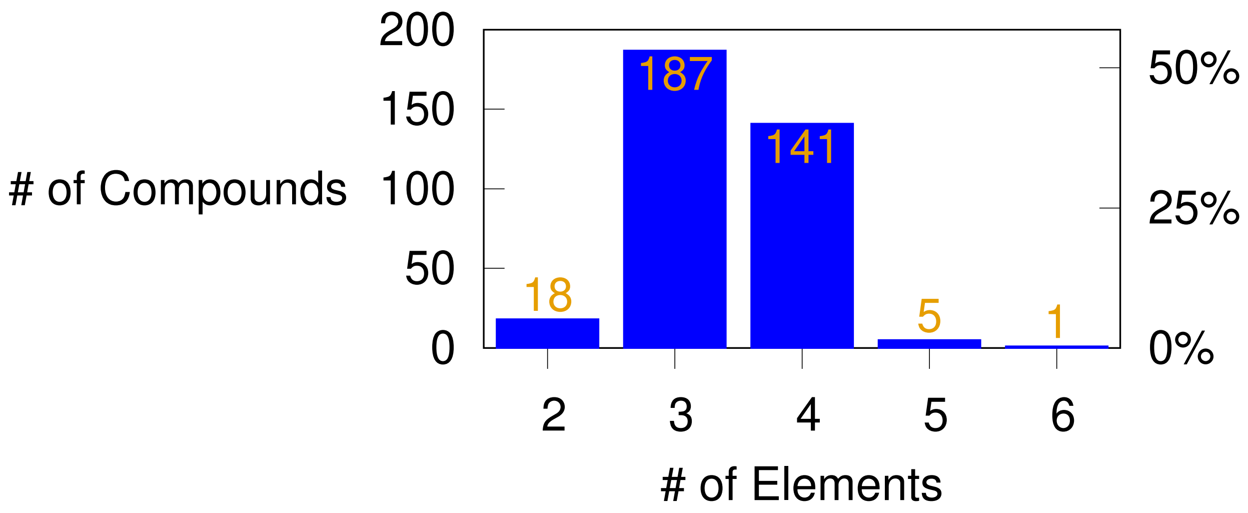


Figure S1: Distribution of the 352 compounds in terms of the number of constituent elements.

As shown in Fig. S1, most of the compounds are ternary or quaternary. The binary compounds are $(As/Sb/Bi)_2(S/Se/Te)_3$; the quinary compounds are $Pb_4As_2S_6ICl$, $AlSb_2Te_2BrCl_4$, $Cs_2CeAsS_3Cl_2$, $H_6C_3BiN_3S_6$, and $Cu_2AgPbBiS_4$; and the six-component compound is $Cs_2NaC_6BiN_6S_6$.

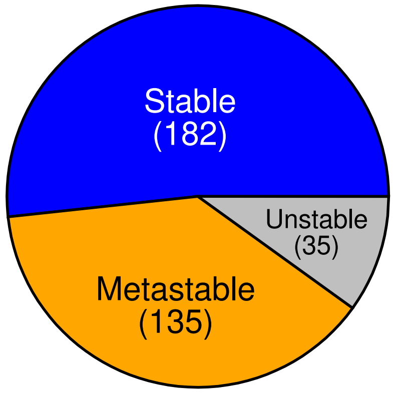


Figure S2: Distribution of the 352 compounds in terms of which are thermodynamically stable (on the convex hull), metastable (within 25 meV/atom of the convex hull), or unstable (otherwise).

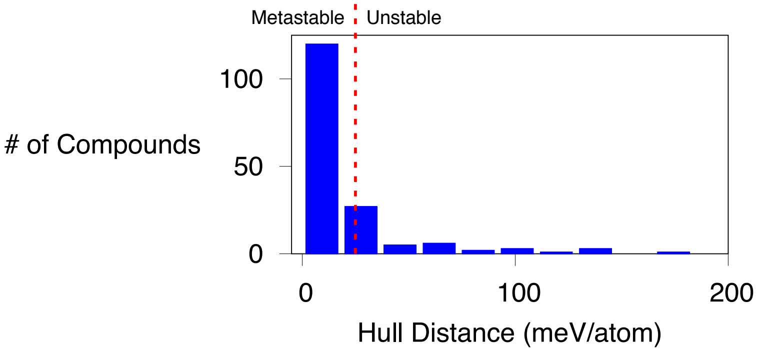


Figure S3: Distribution of hull distance, the energy above the convex hull, for the metastable and unstable compounds.

As shown in Fig. S2, most of the compounds are on or close to the convex hull (thermodynamic ground state). The distribution of energy above the convex hull (ignoring the stable compounds), shown in Fig. S3, sharply drops off with increasing energy. We note that two outliers are not shown: a high-pressure $Bi_2Te_3$ phase (250 meV/atom)[S1] and a $TlSbSe_2$ phase (367 meV/atom) whose refinement[S2] has been criticized.[S3]

The vast majority (325) of the 352 compounds come from the ICSD, with many corresponding structural prototypes. There are 68 unique ICSD prototype labels representing 173 of the ICSD compounds. The five most represented prototypes are:

1. $Na_3AsS_3$-type: 13 compounds (e.g., $Tl_3SbSe_3$)

2. $CaFe_2O_4$-type: 9 compounds (e.g., $Bi_2PbS_4$)

3. $PbCl_2$-type: 8 compounds (e.g., BiSeBr)

4. $NaCrS_2$-type: 8 compounds (e.g., $TlSbTe_2$)

5. $AgBiSe_2$-type: 7 compounds (e.g., $GeSb_4Te_7$)

No single chemical class dominates, but Sb and Bi sulfides are the most prevalent, as shown in Fig. S4. The majority of the compounds contain only a single chalcogen and single pnictogen, but there are a few exceptions: three contain multiple pnictogens

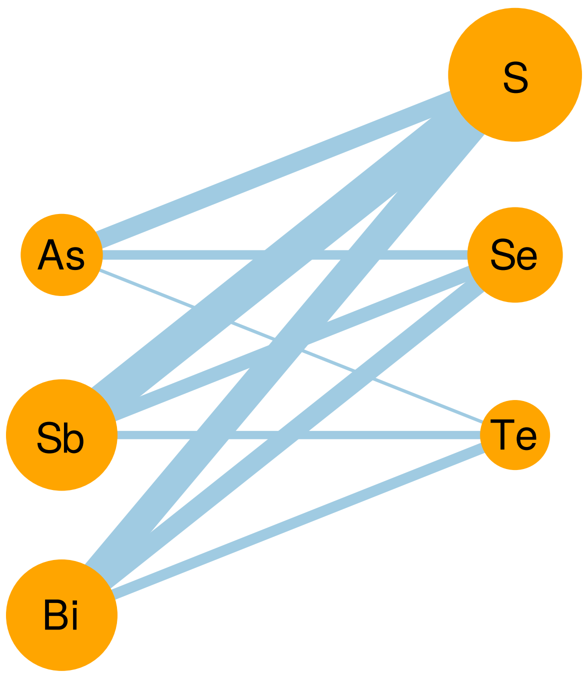


Figure S4: Network illustrating the relative occurrence of different chalcogen and pnictogen cation elements among the 352 compounds. The size of each node is proportional to the number of compounds containing the corresponding element, and the thickness of each edge is proportional to the number of compounds containing both corresponding elements.

($FeBiSbS_4$, $K_3BiAs_6Se_{12}$, and $Ag_3BiSb_2S_6$) and 7 contain multiple chalcogens ($Bi_2STe_2$, $Bi_2SeTe_2$, $Bi_2Se_2Te$, $Sb_2SeTe_2$, $Sb_2Se_2Te$, and $Bi_{14}Te_{13}S_8$).

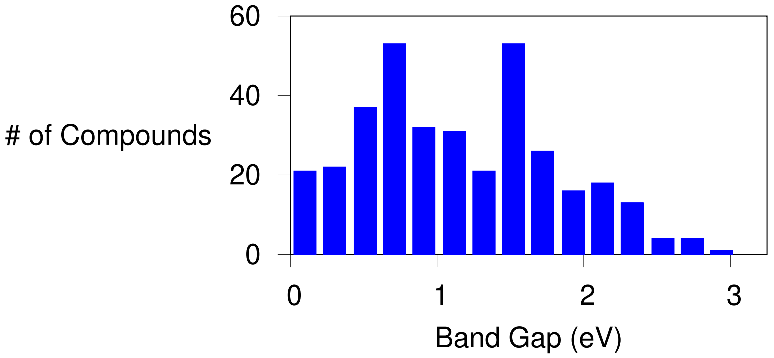


Figure S5: Distribution of electronic band gap for the 352 compounds.

All but 19 of the compounds are semiconductors and insulators, as desired. The distribution of electronic band gaps, shown in Fig. S5, indicates a wide range of band gaps between 0 and 3 eV.

# Details about screening criteria

For the crystal structure criterion, we consider the set of anion (S, Se, or Te) atoms closer to a lone pair (LP) cation atom than any non-anion atom, ignoring atoms $\geq 50\%$ beyond the nearest neighbor in distance. We require that for every site of any pnictogen LP cation element (As, Sb, or Bi):

1. The size of this set is at least 3 (i.e., the LP cation is coordinated by anions with coordination number $\geq 3$), and

2. At least 1 of the corresponding bond angles is less than 109.5° (to enable computation of $\overline{\alpha}^{(s)}$).

For the electron counting criterion, we employ a composition-based algorithm based on common oxidation states, similar to that of our previous work.[S4] We consider each combination of the relevant oxidation states, only allowing a single oxidation state per element. If

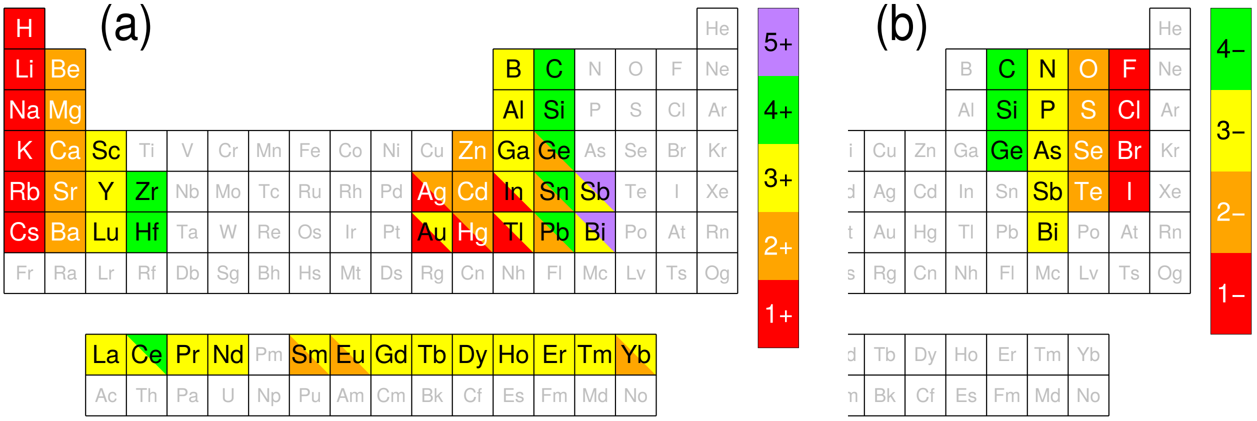


Figure S6: Common oxidation states considered for (a) cations and (b) anions. For cations with two common oxidation states, the oxidation states are indicated by the two colored triangles. For transition metal elements for which no common oxidation state is prescribed (e.g., Cu), the oxidation state can be determined via charge neutrality, as discussed in the text.

there is a single transition metal element with no prescribed common oxidation state(s), we choose the value that would lead to charge neutrality, unless it is non-positive or corresponds to a loss of more than its number of valence electrons. In the end, we keep a compound if any desired charge balanced combination exists. The common oxidation states considered are shown in Fig. S6.

Related to our electron counting algorithm, we note that most compounds with effective coordination number $\sim 3$ and $\langle\overline{\alpha}\rangle \approx 109.5°$ in the main text (e.g., $KAg_2SbS_4$) should be considered false positives related to considering $Ag^{2+}$ (e.g., yielding $Sb^{3+}$ for $KAg_2SbS_4$) in addition to the more likely $Ag^{+}$ (e.g., yielding $Sb^{5+}$ for $KAg_2SbS_4$).

# Dynamical instability of $Cu_2AgBiPbS_4$

The phonons of $Cu_2AgBiPbS_4$ (computed using a 180-atom supercell of the primitive cell) are shown in Fig. S7 and indicate a dynamical instability at finite wavevector.

$Cu_2AgBiPbS_4$ contains partial occupancy of the Cu2 (trigonal planar) sites, with one site having 31% occupancy (Cu2a) and one having 67% occupancy (Cu2b), as shown in

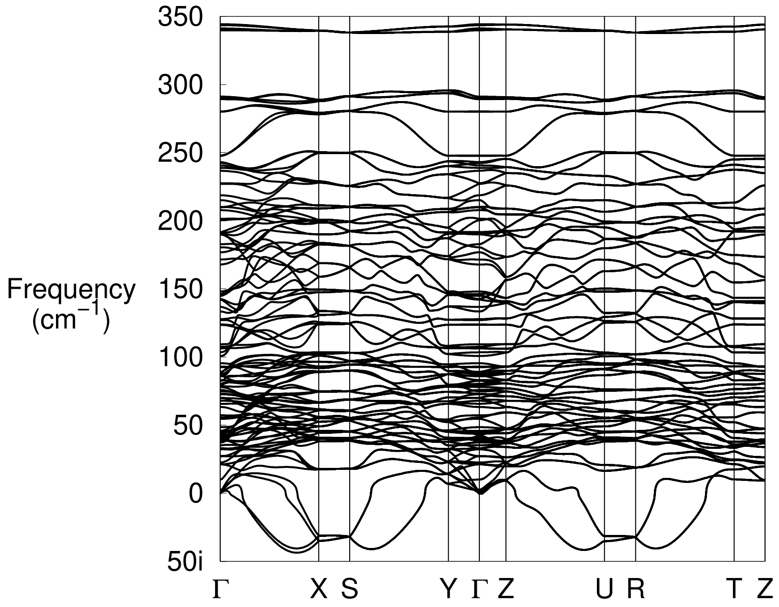


Figure S7: Phonon dispersion for the primitive cell phase of $Cu_2AgBiPbS_4$.

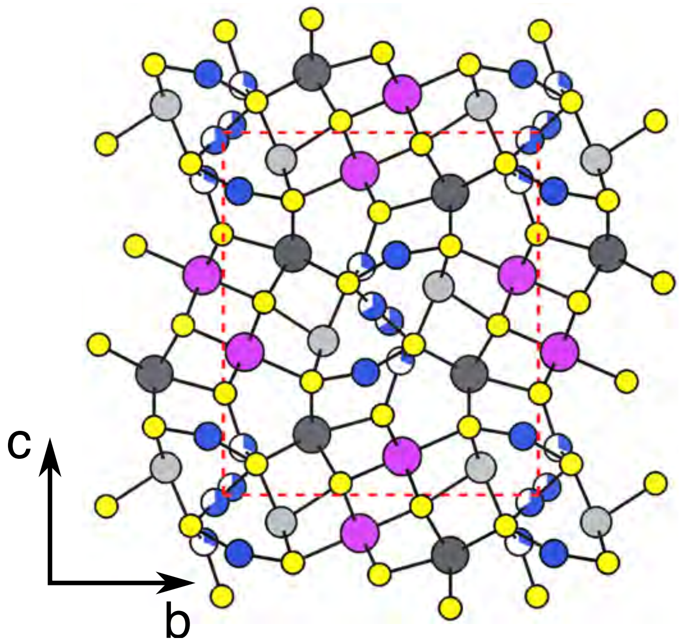


Figure S8: Experimental crystal structure of $Cu_2AgBiPbS_4$. Blue, silver, purple, dark grey, and yellow circles indicate the Cu, Ag, Bi, Pb, and S atoms, respectively. Each atom on a partially-occupied Cu2a and Cu2b site is indicated by a "pie chart" whose blue fraction indicates the occupancy. The unit cell is shown as the dashed red line.

the experimental crystal structure in Fig. S8.[S5] This partial occupancy is ignored by the OQMD:[S6] the $Cu_2AgBiPbS_4$ structure (before structural relaxation) is based on completely occupying the Cu2b site and completely deoccupying the Cu2a site. Therefore, it is perhaps not surprising that the structure from the OQMD is dynamically unstable.

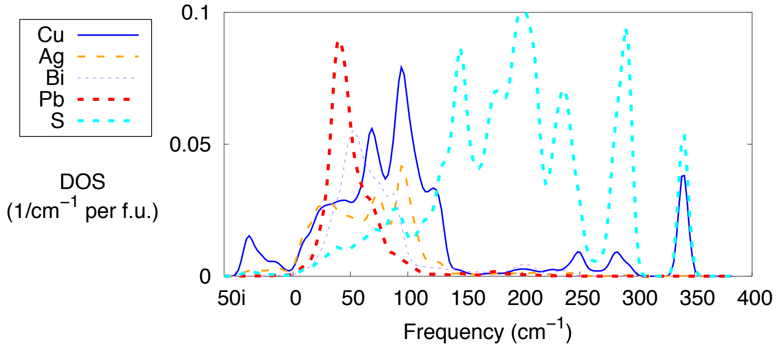


Figure S9: Atom-projected phonon density of states of the primitive cell phase of $Cu_2AgBiPbS_4$.

Indeed, the projected phonon density of states shown in Fig. S9 indicates that the unstable modes correspond almost exclusively to Cu (the trigonal planar Cu in particular) motion. This can also be seen in the included video of the soft mode with the most imaginary frequency at the X point (`Cu2AgBiPbS4_soft_x.gif`). Therefore, the dynamical instability can be viewed as an artifact of the treatment of the Cu partial occupancy.

We generate a doubled (along the $x$ direction) supercell of $Cu_2AgBiPbS_4$, such that it is commensurate with the X point of the Brillouin zone, and nudge the structure with a small amplitude of the soft mode with the most imaginary frequency at X. Relaxing the structure, we find a small (3 meV/atom) energy lowering. As discussed in the main text, the phonon frequencies of this phase are all real, indicating dynamical stability. Therefore, we use this phase as an approximant to the actual system in order to enable study of the lattice dynamical properties. We note that the structural relaxation yields a small monoclinic distortion ($\gamma = 90.6°$), but we still use a primitive orthorhombic high-symmetry path in momentum space for convenience and comparison purposes.

# Acoustic branch definitions for $Cu_2AgBiPbS_4$ and $MnTl_2As_2S_5$

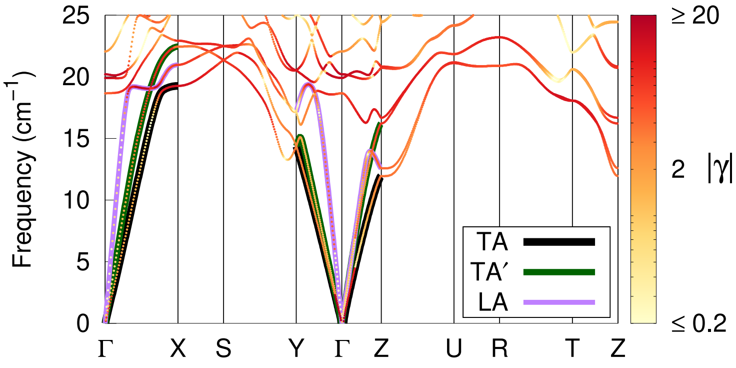


Figure S10: Acoustic branch definitions for $Cu_2AgBiPbS_4$.

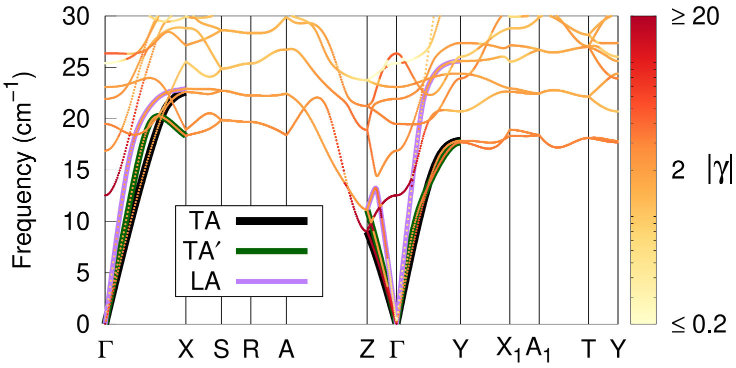


Figure S11: Acoustic branch definitions for $MnTl_2As_2S_5$.

Our definitions for the two transverse acoustic (TA and TA′) and longitudinal acoustic (LA) branches, used for the lattice thermal conductivity ($\kappa_L$) calculations in the main text, are indicated in Figs. S10 and S11.

# Phonon mode visualizations

Included in the Supporting Information are videos of various phonon modes of interest for dynamically stable $Cu_2AgBiPbS_4$ and $MnTl_2As_2S_5$:

- `Cu2AgBiPbS4_gamma_lowest_optical.gif`: lowest optical mode at Γ for $Cu_2AgBiPbS_4$

- `Cu2AgBiPbS4_half_{x,y,z}_{ta,tap,la}.gif`: (TA, TA′, LA) mode at 1/2 (X, Y, Z) for $Cu_2AgBiPbS_4$
- `MnTl2As2S5_gamma_lowest_optical.gif`: lowest optical mode at Γ for $MnTl_2As_2S_5$
- `MnTl2As2S5_half_{x,y,z}_{ta,tap,la}.gif`: (TA, TA′, LA) mode at 1/2 (X, Y, Z) for $MnTl_2As_2S_5$

# Electronic properties of $Cu_2AgBiPbS_4$ and $MnTl_2As_2S_5$

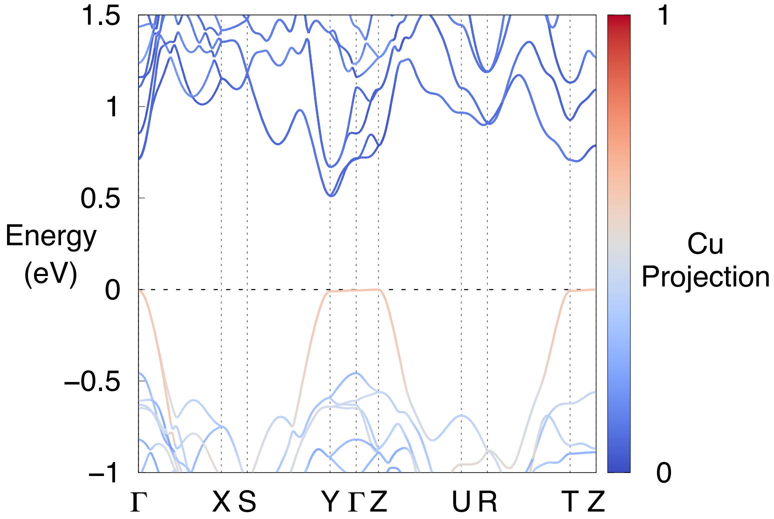


Figure S12: Electronic band structure of $Cu_2AgBiPbS_4$ (primitive cell phase). The color indicates the projection on Cu atoms. The zero of energy is set to the valence band maximum.

The electronic band structure of the (dynamically unstable) primitive cell phase of $Cu_2AgBiPbS_4$ is shown in Fig. S12, indicating it is a semiconductor with a band gap of approximately 0.5 eV. As shown in the projected electronic density of states in Fig. S13, the valence band is composed of Cu states, whereas the conduction band has contributions from various elements. The valence band is flat along the $y$ and $z$ directions, whereas it is dispersive along the $x$ direction, related to Cu–S connectivity along this direction.

The dynamically stable $Cu_2AgBiPbS_4$ phase has a significantly larger electronic band gap ($\sim$ 0.9 eV), as shown in the projected electronic density of states in Fig. S14. In order

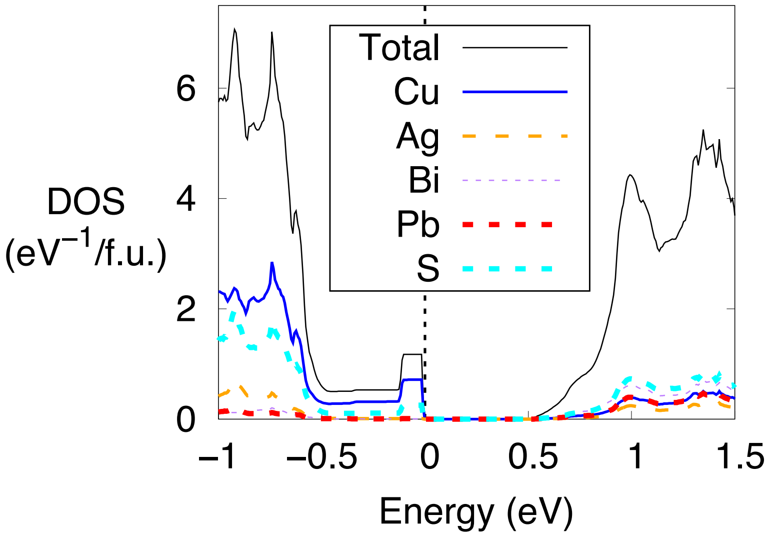


Figure S13: Total and atom-projected electronic density of states of dynamically unstable $Cu_2AgBiPbS_4$.

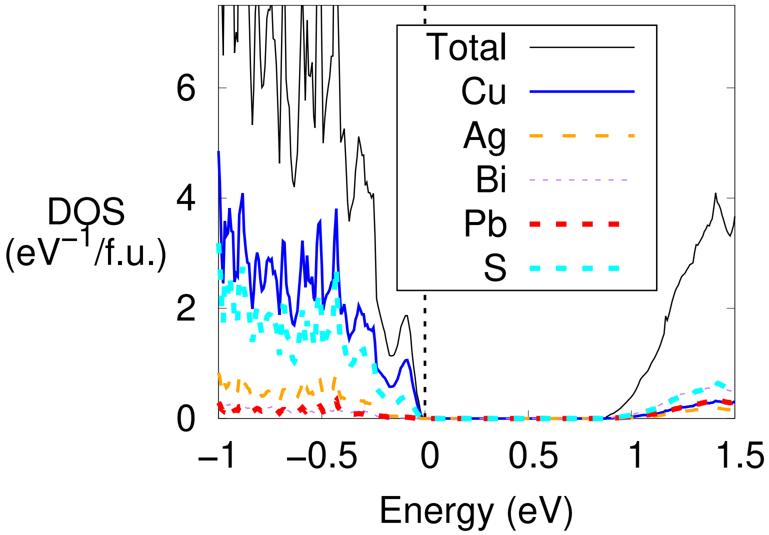


Figure S14: Total and atom-projected electronic density of states of dynamically stable $Cu_2AgBiPbS_4$.

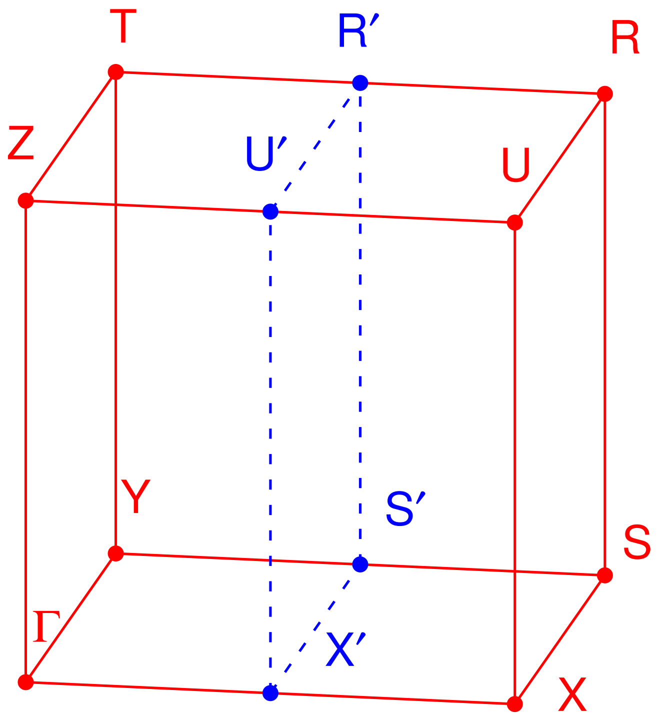


Figure S15: Irreducible Brillouin zone of the primitive cell of $Cu_2AgBiPbS_4$, shown in red. The unit cell of the dynamically stable $Cu_2AgBiPbS_4$ phase, which is doubled along the $x$ direction, is exactly half as large (before relaxing the lattice vectors), and yields band folding across the plane containing the X′, S′, U′, and R′ high-symmetry points, shown in blue.

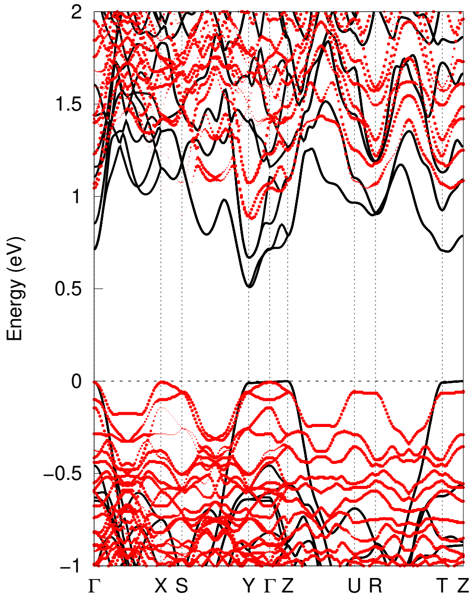


Figure S16: Unfolded electronic band structure of the dynamically stable $Cu_2AgBiPbS_4$ phase (red points). The band structure of the primitive cell phase (black lines) is shown for comparison. The zero of energy is set to the valence band maximum.

to understand the effect on the electronic band structure, we perform band unfolding using the BANDUP code.[S7] The two irreducible Brillouin zones are shown in Fig. S15 and the unfolded band structure is shown in Fig. S16. In the dynamically stable phase, new valence band maxima near the band edge emerge near the X, S, U, and R points. Similarly, in the conduction band region, the band minima near R and T (for example) become significantly closer to the minimum at Y forming the band edge.

$MnTl_2As_2S_5$ contains one-dimensional chains of edge-sharing octahedral $MnS_6$ units. Given the $d^5$ configuration of Mn, we include spin polarization and test several magnetic ordering. We find the ground state is antiferromagnetic with anti-aligned moments for the first (within the chain) and second (between chains) nearest neighbor Mn sites. However, given the ferromagnetic state is only 2 meV/atom higher in energy, we employ ferromagnetic ordering for convenience. As shown in Fig. S17, $MnTl_2As_2S_5$ is a magnetic semiconductor with a band gap of 0.6 eV. As shown in the projected electronic density of states in Fig. S18, the valence band is composed of Mn and S states, whereas the conduction band is composed

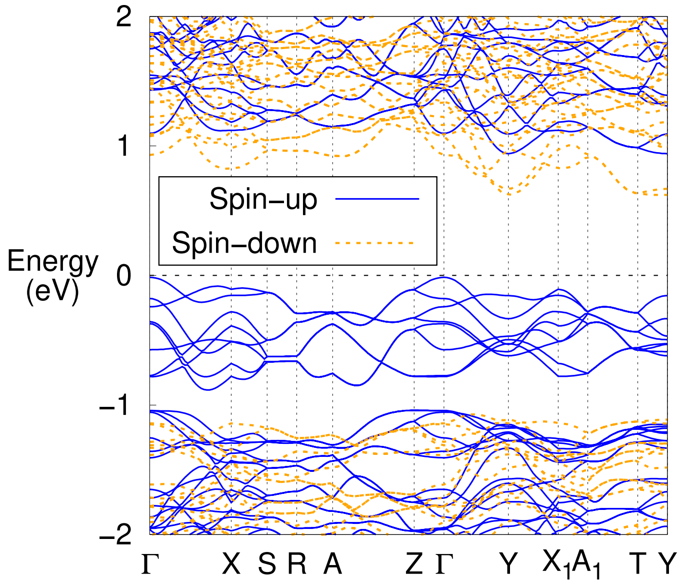


Figure S17: Electronic band structure of $MnTl_2As_2S_5$. The zero of energy is set to the valence band maximum.

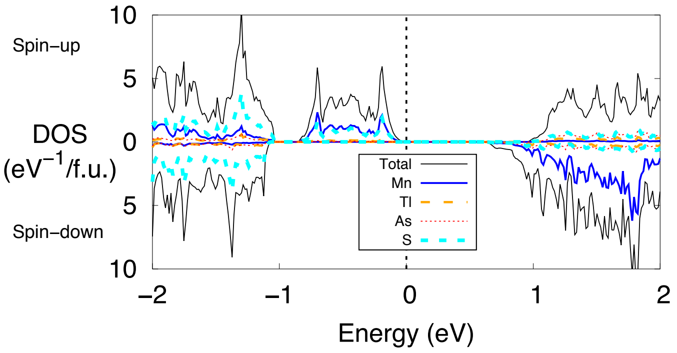


Figure S18: Total and atom-projected electronic density of states of $MnTl_2As_2S_5$.

primarily of Mn states.

# Investigation of coupling between LP states and anharmonic phonons

Here, we investigate whether the LP couples strongly with anharmonic modes in $Cu_2AgBiPbS_4$ and $MnTl_2As_2S_5$. If so, this could suggest the LP is related to the ultralow $\kappa_L$. To assess this, we freeze in particularly anharmonic acoustic modes (considering acoustic modes since these contribute to our computed $\kappa_L$): we choose the $TA_x$ mode for $Cu_2AgBiPbS_4$ and the $TA_z$ mode for $MnTl_2As_2S_5$, at the zone boundary in both cases. The amplitude is chosen such that the root-mean-square atomic displacement is $\approx 0.15$ Å in both cases. We assess whether the parts of the density of states or electronic localization function (ELF) associated with the LP change significantly with respect to the unperturbed system.

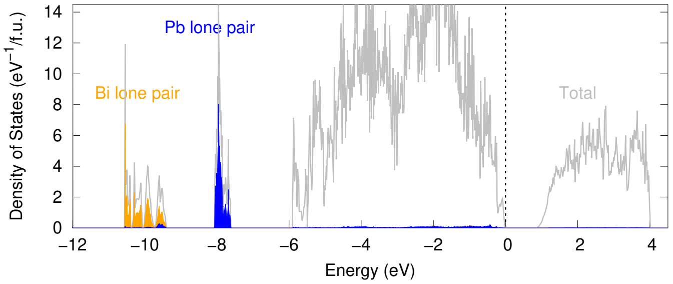


Figure S19: Total and LP-projected electronic density of states of pristine $Cu_2AgBiPbS_4$.

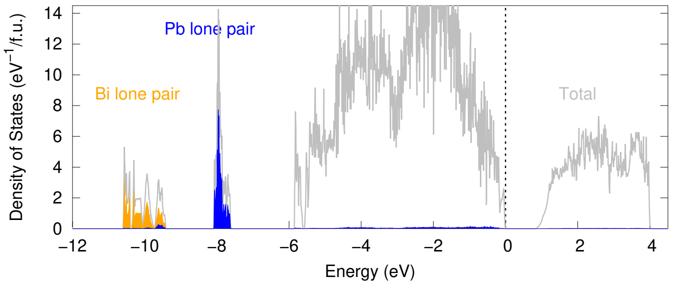


Figure S20: Total and LP-projected electronic density of states of perturbed $Cu_2AgBiPbS_4$.

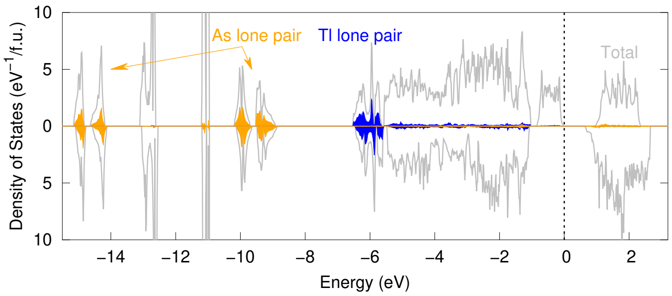


Figure S21: Total and LP-projected electronic density of states of pristine $MnTl_2As_2S_5$.

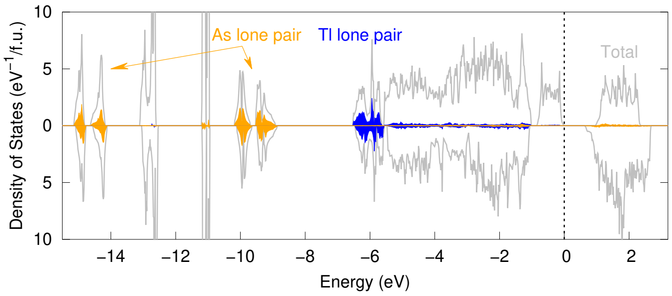


Figure S22: Total and LP-projected electronic density of states of perturbed $MnTl_2As_2S_5$.

We first consider the electronic density of states. Figure S19 (Fig. S20) shows the LP projected electronic density of states for the pristine (perturbed) $Cu_2AgBiPbS_4$. The corresponding plots for $MnTl_2As_2S_5$ are shown in Fig. S21 (pristine) and Fig. S22 (perturbed). In both cases, the LP states are deeply bound and far from the valence band edge, and the perturbation of the anharmonic acoustic mode does not lead to a significant difference in the LP density of states.

Next, we consider the ELF. The ELF for $Cu_2AgBiPbS_4$ and $MnTl_2As_2S_5$ are shown in Figs. S23 and S24, respectively. The Bi LP, which is centered around Bi, is not particularly localized, and an isosurface of as low as 0.45 is needed for visualization. For $MnTl_2As_2S_5$, we show the spin-up ELF, but the spin-down ELF looks nearly identical in the region shown (since the spin polarization is only significant near Mn). In this case, the As LP is quite localized (isosurface of 0.85), and it is spatially pointed away from the three As–S bonds.

The difference in ELF (perturbed with respect to pristine) of $Cu_2AgBiPbS_4$ is shown in

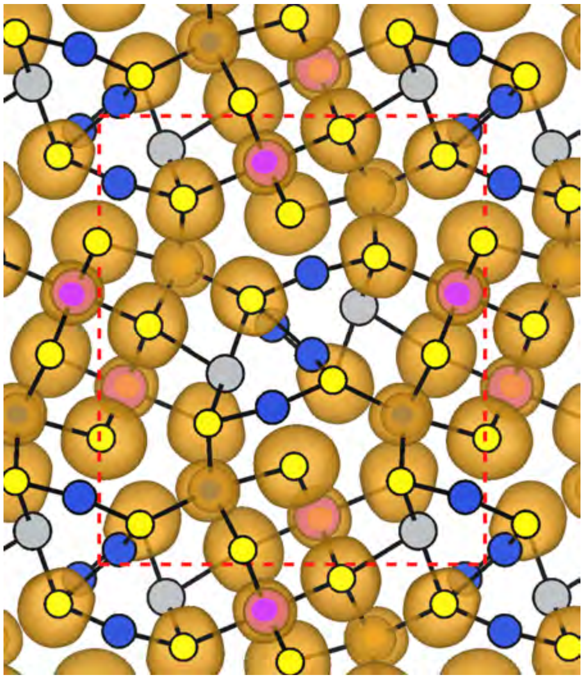

Figure S23: Isosurface (orange) of 0.45 for the electronic localization function of $Cu_2AgBiPbS_4$. Blue, silver, purple, dark grey, and yellow circles indicate the Cu, Ag, Bi, Pb, and S atoms, respectively.

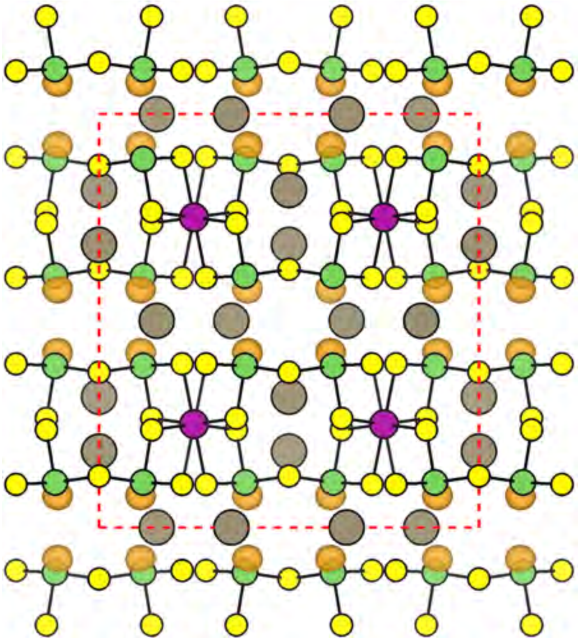

Figure S24: Isosurface (orange) of 0.85 for the spin-up electronic localization function of $MnTl_2As_2S_5$. Purple, dark grey, green, and yellow circles indicate Mn, Tl, As, and S atoms, respectively.

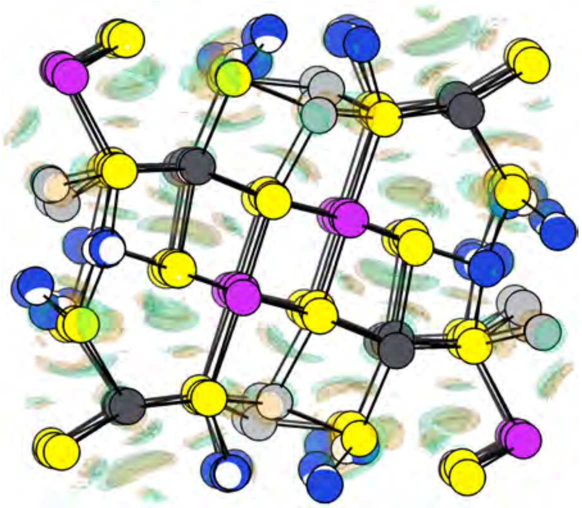

Figure S25: Isosurface of 0.10 for the difference between the perturbed and pristine electronic localization function for $Cu_2AgBiPbS_4$. Positions of the pristine atoms are shown as small white spheres, and the corresponding perturbed atomic positions are shown as larger colored spheres. Blue, silver, purple, dark grey, and yellow correspond to Cu, Ag, Bi, Pb, and S, respectively. The orange (green) components of the isosurface correspond to an increase (decrease) in electronic localization function.

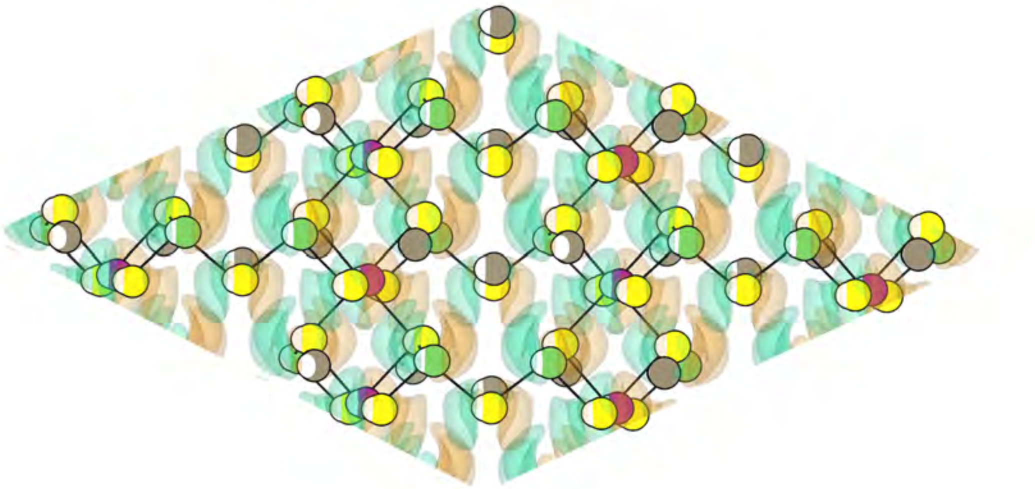

Figure S26: Isosurface of 0.10 for the difference between the perturbed and pristine spin-up electronic localization function for $MnTl_2As_2S_5$. Positions of the pristine atoms are shown as small white spheres, and the corresponding perturbed atomic positions are shown as larger colored spheres. Purple, dark grey, green, and yellow correspond to Mn, Tl, As, and S, respectively. The orange (green) components of the isosurface correspond to an increase (decrease) in electronic localization function.

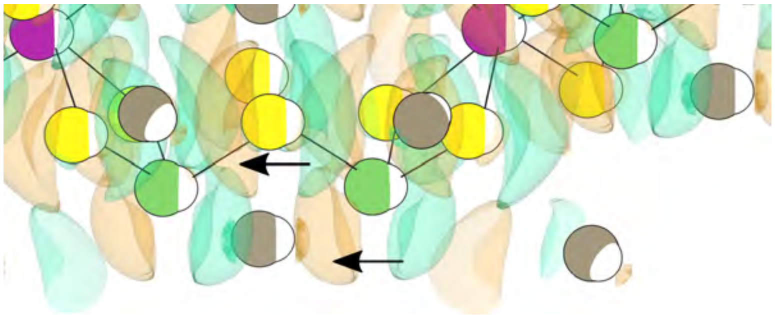

Figure S27: Isosurface of 0.10 for the difference between the perturbed and pristine spin-up electronic localization function for $MnTl_2As_2S_5$. Positions of the pristine atoms are shown as small white spheres, and the corresponding perturbed atomic positions are shown as larger colored spheres. Purple, dark grey, green, and yellow correspond to Mn, Tl, As, and S, respectively. The orange (green) components of the isosurface correspond to an increase (decrease) in electronic localization function. The bottom arrow indicates the movement of the As atom and associated LP, and the top arrow indicates the corresponding movement for the S atom and its $p$ electrons.

Fig. S25. The largest differences in ELF are not in the region near Bi. Two visualizations of the corresponding difference for $MnTl_2As_2S_5$ are shown in Figs. S26 and S27. In this case, the As LP appears to closely track the motion of the As atom.

The anharmonic acoustic phonons do not dramatically impact the LP energies (as captured by the electronic density of states) or the spatial arrangement of the LP (as captured by the ELF). Therefore, as mentioned in the main text, we are unable to find evidence that the presence of the LP, or the LP cation coordination environment, directly causes the ultralow $\kappa_L$ in $Cu_2AgBiPbS_4$ and $MnTl_2As_2S_5$.

# Complete list of 352 compounds

**Table S1: Compound composition; space group (SG); # of primitive cell atoms ($N_{\text{atoms}}$); thermodynamic stability (in meV/atom); ICSD presence, number, and listed prototype (if any); and $\overline{\alpha}$ and effective coordination number (ECoN) data for each constituent pnictogen LP cation element for the 352 compounds passing the initial screening. The 189 compounds determined to be the most promising, based on coordination environment (as discussed in the main text), are listed in bold. The thermodynamic stability is the (positive) energy above the convex hull for metastable/unstable compounds, while for stable compounds it is a negative value indicating the magnitude of formation energy increase for which the compound would no longer be on the convex hull.**

| Composition | SG | $N_{\text{atoms}}$ | Stab. | In ICSD? | ICSD # | Prototype | LP El. | $\langle\overline{\alpha}\rangle$ | $\overline{\alpha}$ | ⟨ECON⟩ | ECoN |
|---|---|---|---|---|---|---|---|---|---|---|---|
| **$As_2S_3$** | $P21/c$ | 20 | 0 | Yes | 25792 | As2S3 | As | 99.0 | 98.5–99.4 | 3.0 | 3.0–3.0 |
| **$As_2S_3$** | $P21/c$ | 20 | -40 | Yes | 15239 | As2S3 | As | 98.9 | 98.5–99.3 | 3.0 | 3.0–3.0 |
| $Sb_2S_3$ | $Pnma$ | 20 | 1 | Yes | 22176 | Sb2S3 | | | | | |
| $Sb_2S_3$ | $Pnma$ | 20 | -285 | Yes | 99797 | Sb2S3 | | | | | |
| $Bi_2S_3$ | $Pnma$ | 20 | -304 | Yes | 30775 | Sb2S3 | | | | | |
| $As_2Se_3$ | $P21/c$ | 20 | -40 | Yes | 2600 | As2S3 | | | | | |
| $As_2Se_3$ | $P21/c$ | 20 | 0 | Yes | 43226 | As2S3 | | | | | |
| $Sb_2Se_3$ | $Pnma$ | 20 | 74 | Yes | 651515 | | | | | | |
| $Sb_2Se_3$ | $Pnma$ | 20 | -226 | Yes | 16680 | Sb2S3 | | | | | |
| $Bi_2Se_3$ | $P42/nmc$ | 40 | 135 | Yes | 617096 | Zn3P2 | | | | | |
| $Bi_2Se_3$ | $Pnma$ | 20 | 20 | Yes | 60205 | Sb2S3 | | | | | |
| **$Bi_2Se_3$** | $R\bar{3}m$ | 5 | -91 | Yes | 20385 | Bi2Te3 | Bi | 89.9 | 89.9–89.9 | 5.7 | 5.7–5.7 |
| **$As_2Te_3$** | $R\bar{3}m$ | 5 | 8 | Yes | 68110 | Bi2Te3 | As | 90.0 | 90.0–90.0 | 5.9 | 5.9–5.9 |
| **$As_2Te_3$** | $C2/m$ | 10 | -15 | Yes | 18208 | Gd2Cl3 | As | 90.3 | 90.0–90.6 | 4.7 | 3.6–5.9 |
| **$Sb_2Te_3$** | $R\bar{3}m$ | 5 | -33 | Yes | 262171 | | Sb | 90.0 | 90.0–90.0 | 5.8 | 5.8–5.8 |
| $Sb_2Te_3$ | $C2/m$ | 10 | 51 | Yes | 262172 | | | | | | |
| **$Bi_2Te_3$** | $R\bar{3}m$ | 5 | -58 | Yes | 15753 | Bi2Te3 | Bi | 90.0 | 90.0–90.0 | 5.8 | 5.8–5.8 |
| **$Bi_2Te_3$** | $R3m$ | 5 | 249 | Yes | 20289 | In2Se3 | Bi | 89.9 | 89.9–90.0 | 5.7 | 5.7–5.7 |
| **$Bi_{14}Te_{13}S_8$** | $P\bar{1}$ | 35 | 14 | Yes | 159356 | Ca.5Ti2P3O12 | Bi | 90.0 | 90.0–90.0 | 5.8 | 5.5–6.1 |
| **$Bi_2Te_2S$** | $R\bar{3}m$ | 5 | -15 | Yes | 26720 | | Bi | 90.0 | 90.0–90.0 | 6.0 | 6.0–6.0 |
| **BiSCl** | $Pnma$ | 12 | -37 | Yes | 25573 | PbCl2 | Bi | 87.8 | 87.8–87.8 | 4.9 | 4.9–4.9 |
| SbSBr | $Pnma$ | 12 | -40 | Yes | 26469 | PbCl2 | | | | | |
| BiSBr | $Pnma$ | 12 | -11 | Yes | 25574 | PbCl2 | | | | | |
| SbSI | $P212121$ | 12 | 1 | Yes | 85298 | SbSI | | | | | |
| SbSI | $P212121$ | 12 | 1 | Yes | 85299 | SbSI | | | | | |
| SbSI | $Pnma$ | 12 | -16 | Yes | 26923 | PbCl2 | | | | | |
| BiSI | $Pnma$ | 12 | 0 | Yes | 23631 | PbCl2 | | | | | |
| **$Cu_6As_4S_9$** | $P1$ | 38 | -14 | Yes | 66660 | | As | 102.6 | 99.9–104.8 | 2.9 | 2.8–2.9 |
| $LiAsS_2$ | $Cc$ | 8 | -15 | Yes | 419061 | | | | | | |
| $LiSbS_2$ | $R\bar{3}$ | 24 | 2 | Yes | 40457 | AgAsS2 | | | | | |
| **$NaAsS_2$** | $P21/c$ | 16 | -48 | Yes | 854 | AsNaS2 | As | 100.5 | 100.5–100.5 | 2.9 | 2.9–2.9 |
| $NaSbS_2$ | $C2/c$ | 8 | -104 | Yes | 43909 | KFeS2 | | | | | |
| $NaSbS_2$ | $C2/m$ | 8 | 19 | Yes | 49016 | | | | | | |
| $KSbS_2$ | $C2/c$ | 8 | -56 | Yes | 60138 | KFeS2 | | | | | |
| $KBiS_2$ | $R\bar{3}m$ | 4 | -119 | No | | | | | | | |
| **$CsAsS_2$** | $P21/c$ | 32 | -130 | No | | | As | 101.1 | 100.0–102.3 | 2.8 | 2.8–2.8 |
| $RbSbS_2$ | $P\bar{1}$ | 16 | -30 | Yes | 56788 | TlSbS2 | | | | | |
| $CsSbS_2$ | $P21/c$ | 16 | -42 | Yes | 653612 | | | | | | |
| **$RbBiS_2$** | $R\bar{3}m$ | 4 | -172 | Yes | 52735 | | Bi | 90.0 | 90.0–90.0 | 6.0 | 6.0–6.0 |

| | | | | | | | | | | | |
|---|---|---|---|---|---|---|---|---|---|---|---|
| $CsBiS_2$ | $P21/c$ | 16 | -70 | Yes | 72975 | | | | | | |
| $AgAsS_2$ | $R\bar{3}$ | 24 | 0 | Yes | 18101 | AgAsS2 | | | | | |
| $CuSbS_2$ | $Pnma$ | 16 | -13 | Yes | 30280 | CuBiS2 | | | | | |
| $CuBiS_2$ | $Pnma$ | 16 | -10 | Yes | 34936 | CuBiS2 | | | | | |
| $AgSbS_2$ | $C2$ | 16 | -7 | Yes | 85130 | | | | | | |
| $AgSbS_2$ | $Cc$ | 16 | 72 | Yes | 16578 | | | | | | |
| $\mathbf{AgBiS_2}$ | $P\bar{3}m1$ | 12 | 17 | Yes | 44340 | AgBiSe2 | Bi | 90.0 | 90.0–90.0 | 6.1 | 6.1–6.1 |
| $TlAsS_2$ | $P21/c$ | 32 | 0 | Yes | 79581 | TlAsS2 | | | | | |
| $TlAsS_2$ | $P21/c$ | 32 | -24 | Yes | 15231 | TlAsS2 | | | | | |
| $TlSbS_2$ | $P\bar{1}$ | 16 | -26 | Yes | 35498 | TlSbS2 | | | | | |
| $\mathbf{TlBiS_2}$ | $R\bar{3}m$ | 4 | -69 | Yes | 166490 | NaCrS2 | Bi | 90.0 | 90.0–90.0 | 6.0 | 6.0–6.0 |
| $\mathbf{Li_3AsS_3}$ | $Pna21$ | 28 | -8 | Yes | 59381 | | As | 102.1 | 102.1–102.1 | 3.0 | 3.0–3.0 |
| $\mathbf{Na_3AsS_3}$ | $P213$ | 28 | -53 | Yes | 645 | Na3AsS3 | As | 102.2 | 102.2–102.2 | 3.0 | 3.0–3.0 |
| $\mathbf{K_3AsS_3}$ | $P213$ | 28 | -83 | Yes | 610764 | Na3AsS3 | As | 103.9 | 103.9–103.9 | 3.0 | 3.0–3.0 |
| $Cu_3AsS_3$ | $I\bar{4}3m$ | 28 | 31 | Yes | 33588 | Cu3SbS3 | | | | | |
| $\mathbf{Ag_3AsS_3}$ | $C2/c$ | 28 | -16 | Yes | 36352 | Xanthoconite | As | 99.9 | 99.9–99.9 | 3.0 | 3.0–3.0 |
| $\mathbf{Ag_3AsS_3}$ | $R3c$ | 14 | 4 | Yes | 27841 | Proustite | As | 98.9 | 98.9–98.9 | 3.0 | 3.0–3.0 |
| $\mathbf{Ag_3AsS_3}$ | $R3c$ | 14 | 11 | Yes | 32652 | Proustite | As | 98.8 | 98.8–98.8 | 3.0 | 3.0–3.0 |
| $\mathbf{Cu_3SbS_3}$ | $P21/c$ | 56 | 24 | Yes | 74901 | | Sb | 97.3 | 97.1–97.4 | 3.0 | 3.0–3.0 |
| $\mathbf{Cu_3SbS_3}$ | $P212121$ | 28 | 22 | Yes | 403113 | | Sb | 98.4 | 98.4–98.4 | 3.1 | 3.1–3.1 |
| $Cu_3SbS_3$ | $I\bar{4}3m$ | 28 | 38 | Yes | 31113 | Cu3SbS3 | | | | | |
| $Ag_3SbS_3$ | $P21/c$ | 28 | -4 | Yes | 33714 | | | | | | |
| $Ag_3SbS_3$ | $R3c$ | 14 | 3 | Yes | 27842 | Proustite | | | | | |
| $Ag_3SbS_3$ | $R3c$ | 14 | 7 | Yes | 32653 | Proustite | | | | | |
| $Cu_3BiS_3$ | $P212121$ | 28 | 15 | Yes | 14305 | Cu3BiS3 | | | | | |
| $\mathbf{Tl_3AsS_3}$ | $Pbca$ | 56 | -21 | Yes | 79580 | | As | 101.9 | 101.9–101.9 | 3.0 | 3.0–3.0 |
| $\mathbf{Tl_3AsS_3}$ | $R3m$ | 7 | 11 | Yes | 611332 | | As | 102.8 | 102.8–102.8 | 3.0 | 3.0–3.0 |
| $\mathbf{Tl_3SbS_3}$ | $R3m$ | 7 | -0 | Yes | 48133 | | Sb | 99.4 | 99.4–99.4 | 3.0 | 3.0–3.0 |
| $\mathbf{Pb_3Bi_2S_6}$ | $C2/m$ | 22 | -3 | Yes | 92981 | | Bi | 90.0 | 90.0–90.0 | 5.4 | 5.4–5.4 |
| $\mathbf{Pb_3Bi_2S_6}$ | $Cmcm$ | 22 | 5 | Yes | 246062 | | Bi | 90.0 | 90.0–90.0 | 5.3 | 5.3–5.3 |
| $Ca_2Sb_2S_5$ | $P21/c$ | 36 | 0 | Yes | 201044 | | | | | | |
| $\mathbf{Ba_2As_2S_5}$ | $Pca21$ | 72 | -101 | Yes | 37334 | | As | 97.7 | 90.6–101.5 | 3.1 | 2.9–3.2 |
| $Sn_2Sb_2S_5$ | $Pnma$ | 36 | 18 | Yes | 35641 | Pb2Sb2S5 | | | | | |
| $Pb_2Sb_2S_5$ | $Pnma$ | 36 | 11 | Yes | 35640 | Pb2Sb2S5 | | | | | |
| $K_2Sb_4S_7$ | $C2/c$ | 26 | 1 | Yes | 25329 | | | | | | |
| $Rb_2Sb_4S_7$ | $P\bar{1}$ | 26 | -16 | Yes | 2194 | | | | | | |
| $Rb_2Sb_4S_7$ | $P21/c$ | 26 | 11 | Yes | 64673 | | | | | | |
| $\mathbf{Pb_9As_4S_{15}}$ | $R3m$ | 28 | -1 | Yes | 18097 | | As | 99.5 | 99.3–99.5 | 3.0 | 3.0–3.0 |
| $Sr_3Sb_4S_9$ | $Pna21$ | 64 | -19 | Yes | 201400 | | | | | | |
| $Yb_3Sb_4S_9$ | $Pnma$ | 64 | 32 | Yes | 600822 | | | | | | |
| $\mathbf{Ag_3Bi_7S_{12}}$ | $C2/m$ | 22 | 6 | Yes | 100734 | | Bi | 87.2 | 80.2–90.0 | 5.5 | 4.8–6.0 |
| $Ag_5SbS_4$ | $Cmc21$ | 20 | 15 | Yes | 16987 | Ag5SbS4 | | | | | |
| $Pb_5Sb_8S_{17}$ | $C2/c$ | 60 | -4 | Yes | 23569 | Pb5b8S17 | | | | | |
| $\mathbf{BaBi_2S_4}$ | $P63/m$ | 84 | -43 | Yes | 35632 | | Bi | 90.0 | 89.9–90.0 | 4.8 | 3.9–5.4 |
| $EuBi_2S_4$ | $Pnma$ | 28 | 0 | Yes | 616653 | | | | | | |
| $EuBi_2S_4$ | $Pnma$ | 28 | -3 | Yes | 600801 | | | | | | |
| $YbBi_2S_4$ | $Pnma$ | 28 | 35 | Yes | 600812 | CaFe2O4 | | | | | |
| $\mathbf{HgBi_2S_4}$ | $C2/m$ | 14 | -15 | Yes | 14189 | HgBi2S4 | Bi | 85.2 | 80.5–90.0 | 5.1 | 4.9–5.4 |
| $PbBi_2S_4$ | $Pnma$ | 28 | 4 | Yes | 23905 | CaFe2O4 | | | | | |
| $BaSb_2S_4$ | $P21/c$ | 56 | -62 | Yes | 38372 | | | | | | |
| $\mathbf{EuSb_2S_4}$ | $Pnma$ | 28 | 25 | Yes | 631617 | CaFe2O4 | Sb | 84.5 | 78.9–90.0 | 4.7 | 3.9–5.5 |
| $\mathbf{YbSb_2S_4}$ | $Pnma$ | 28 | 58 | Yes | 600800 | CaFe2O4 | Sb | 84.5 | 79.0–90.1 | 4.9 | 4.0–5.8 |
| $MnSb_2S_4$ | $C2/m$ | 14 | -7 | Yes | 411178 | HgBi2S4 | | | | | |
| $MnSb_2S_4$ | $Pnma$ | 28 | 21 | Yes | 56379 | CaFe2O4 | | | | | |
| $FeSb_2S_4$ | $Pnma$ | 28 | 140 | Yes | 16908 | CaFe2O4 | | | | | |
| $PbAs_2S_4$ | $Pnma$ | 28 | 29 | Yes | 24449 | | | | | | |

| | | | | | | | | | | | |
|---|---|---|---|---|---|---|---|---|---|---|---|
| $PbAs_2S_4$ | $Pnma$ | 28 | 28 | Yes | 15464 | | | | | | |
| $\mathbf{KBi_3S_5}$ | $Pnma$ | 40 | -4 | Yes | 79200 | | Bi | 90.0 | 89.9–90.0 | 5.6 | 5.5–5.8 |
| $\mathbf{RbBi_3S_5}$ | $Pnnm$ | 36 | 130 | Yes | 654071 | | Bi | 90.0 | 90.0–90.2 | 5.5 | 4.8–5.9 |
| $\mathbf{CsBi_3S_5}$ | $Pnma$ | 36 | -46 | Yes | 200794 | | Bi | 89.9 | 89.8–90.0 | 5.2 | 4.7–6.0 |
| $\mathbf{AgBi_3S_5}$ | $C2/m$ | 18 | -7 | Yes | 200110 | AgBi3S5 | Bi | 86.7 | 80.3–89.9 | 5.4 | 4.8–5.8 |
| $TlSb_3S_5$ | $P21/c$ | 36 | 4 | Yes | 17058 | | | | | | |
| $CrSbS_3$ | $Pnma$ | 20 | -12 | Yes | 74601 | NH4CdCl3/Sn2S3 | | | | | |
| $InSbS_3$ | $Pnma$ | 20 | -3 | Yes | 300207 | NH4CdCl3/Sn2S3 | | | | | |
| $\mathbf{InBiS_3}$ | $Pnma$ | 20 | -2 | No | | | Bi | 84.3 | 84.3–84.3 | 4.7 | 4.7–4.7 |
| $In_5Bi_3S_{12}$ | $C2/m$ | 40 | 13 | Yes | 23315 | | | | | | |
| $In_4Bi_2S_9$ | $P21/m$ | 30 | 6 | Yes | 2839 | Ho2S3 | | | | | |
| $SnSb_4S_7$ | $P21/m$ | 24 | 7 | Yes | 169941 | | | | | | |
| $KSb_5S_8$ | $Pc$ | 56 | 1 | Yes | 410178 | | | | | | |
| $TlSb_5S_8$ | $Pc$ | 56 | 4 | Yes | 100291 | TlSb5O8 | | | | | |
| $\mathbf{Sb_2TeSe_2}$ | $R3m$ | 5 | 2 | Yes | 60963 | | Sb | 90.0 | 90.0–90.0 | 5.9 | 5.8–6.0 |
| $\mathbf{Sb_2TeSe_2}$ | $R\bar{3}m$ | 5 | 33 | Yes | 52295 | | Sb | 89.8 | 89.8–89.8 | 5.2 | 5.2–5.2 |
| $\mathbf{Bi_2TeSe_2}$ | $R\bar{3}m$ | 5 | 31 | Yes | 54838 | | Bi | 89.8 | 89.8–89.8 | 5.2 | 5.2–5.2 |
| $\mathbf{Sb_2Te_2Se}$ | $R\bar{3}m$ | 5 | -14 | Yes | 2085 | Bi2Te3 | Sb | 90.0 | 90.0–90.0 | 6.0 | 6.0–6.0 |
| $\mathbf{Bi_2Te_2Se}$ | $R\bar{3}m$ | 5 | -15 | Yes | 43512 | Bi2Te3 | Bi | 90.0 | 90.0–90.0 | 6.0 | 6.0–6.0 |
| $\mathbf{BiSeCl}$ | $Pnma$ | 12 | -22 | Yes | 40862 | PbCl2 | Bi | 89.0 | 89.0–89.0 | 5.4 | 5.4–5.4 |
| $\mathbf{BiSeBr}$ | $Pnma$ | 12 | 5 | Yes | 76649 | PbCl2 | Bi | 88.2 | 88.2–88.2 | 4.8 | 4.8–4.8 |
| $\mathbf{Bi_3Se_4Br}$ | $C2/m$ | 16 | 18 | Yes | 411096 | InSb2S4Cl | Bi | 86.7 | 80.4–91.8 | 4.6 | 4.0–5.0 |
| $SbSeI$ | $Pnma$ | 12 | -17 | Yes | 31292 | PbCl2 | | | | | |
| $BiSeI$ | $Pnma$ | 12 | 12 | Yes | 280311 | | | | | | |
| $LiAsSe_2$ | $Cc$ | 8 | -17 | Yes | 248116 | CeCoC2 | | | | | |
| $LiAsSe_2$ | $P\bar{1}$ | 8 | 13 | Yes | 248118 | | | | | | |
| $NaAsSe_2$ | $Pc$ | 32 | -37 | Yes | 248117 | | | | | | |
| $\mathbf{NaSbSe_2}$ | $R\bar{3}m$ | 4 | -77 | No | | | Sb | 90.0 | 90.0–90.0 | 6.0 | 6.0–6.0 |
| $\mathbf{KAsSe_2}$ | $P1$ | 16 | -37 | Yes | 65297 | KSbSe2 | As | 100.2 | 98.8–101.6 | 2.9 | 2.9–2.9 |
| $\mathbf{RbAsSe_2}$ | $C2/c$ | 32 | -42 | Yes | 65298 | | As | 100.8 | 99.9–101.7 | 2.9 | 2.9–2.9 |
| $KSbSe_2$ | $P1$ | 16 | -25 | Yes | 44678 | KSbSe2 | | | | | |
| $\mathbf{KBiSe_2}$ | $R\bar{3}m$ | 4 | -64 | No | | | Bi | 90.0 | 90.0–90.0 | 6.0 | 6.0–6.0 |
| $\mathbf{CsAsSe_2}$ | $P21/c$ | 32 | -9 | Yes | 171373 | | As | 100.7 | 99.3–102.1 | 2.9 | 2.9–2.9 |
| $\mathbf{CsAsSe_2}$ | $Pbca$ | 32 | 3 | Yes | 65299 | | As | 101.2 | 101.2–101.2 | 2.9 | 2.9–2.9 |
| $CsSbSe_2$ | $P21/c$ | 32 | -35 | Yes | 20773 | | | | | | |
| $\mathbf{CuAsSe_2}$ | $R3m$ | 4 | 106 | Yes | 42884 | | As | 102.4 | 102.4–102.4 | 3.9 | 3.9–3.9 |
| $\mathbf{AgAsSe_2}$ | $R\bar{3}m$ | 4 | 20 | Yes | 20087 | NaCrS2 | As | 90.0 | 90.0–90.0 | 6.0 | 6.0–6.0 |
| $CuSbSe_2$ | $Pnma$ | 16 | -7 | Yes | 30358 | CuBiS2 | | | | | |
| $CuBiSe_2$ | $Pnma$ | 16 | 20 | No | | | | | | | |
| $\mathbf{AgBiSe_2}$ | $R\bar{3}m$ | 4 | -4 | Yes | 26518 | NaCrS2 | Bi | 90.0 | 90.0–90.0 | 6.1 | 6.1–6.1 |
| $\mathbf{AgBiSe_2}$ | $P\bar{3}m1$ | 12 | 0 | Yes | 26519 | AgBiSe2 | Bi | 90.0 | 90.0–90.0 | 6.1 | 6.1–6.1 |
| $TlSbSe_2$ | $P21$ | 16 | -14 | Yes | 36537 | | | | | | |
| $\mathbf{TlSbSe_2}$ | $Cmmm$ | 4 | 367 | Yes | 20374 | TlSbSe2 | Sb | 90.0 | 90.0–90.0 | 7.8 | 7.8–7.8 |
| $\mathbf{TlBiSe_2}$ | $R\bar{3}m$ | 4 | -97 | Yes | 43314 | NaCrS2 | Bi | 90.0 | 90.0–90.0 | 6.0 | 6.0–6.0 |
| $\mathbf{Na_3AsSe_3}$ | $P213$ | 28 | -30 | Yes | 50491 | | As | 102.5 | 102.5–102.5 | 3.0 | 3.0–3.0 |
| $\mathbf{K_3AsSe_3}$ | $P213$ | 28 | -96 | Yes | 50492 | | As | 104.3 | 104.3–104.3 | 3.0 | 3.0–3.0 |
| $\mathbf{K_3SbSe_3}$ | $P213$ | 28 | -91 | Yes | 89607 | Na3AsS3 | Sb | 102.2 | 102.2–102.2 | 3.0 | 3.0–3.0 |
| $\mathbf{K_3BiSe_3}$ | $P213$ | 28 | -28 | Yes | 78841 | Na3AsS3 | Bi | 101.2 | 101.2–101.2 | 3.0 | 3.0–3.0 |
| $\mathbf{Rb_3SbSe_3}$ | $P213$ | 28 | -92 | Yes | 89608 | Na3AsS3 | Sb | 102.6 | 102.6–102.6 | 3.0 | 3.0–3.0 |
| $\mathbf{Cs_3SbSe_3}$ | $P213$ | 28 | -107 | Yes | 89609 | Na3AsS3 | Sb | 103.7 | 103.7–103.7 | 3.0 | 3.0–3.0 |
| $\mathbf{Rb_3BiSe_3}$ | $P213$ | 28 | -82 | Yes | 85411 | Na3AsS3 | Bi | 102.3 | 102.3–102.3 | 3.0 | 3.0–3.0 |
| $\mathbf{Cs_3BiSe_3}$ | $P213$ | 28 | -133 | Yes | 85410 | Na3AsS3 | Bi | 103.1 | 103.1–103.1 | 3.0 | 3.0–3.0 |
| $\mathbf{Ag_3AsSe_3}$ | $R3c$ | 14 | -6 | Yes | 2426 | Proustite | As | 97.2 | 97.2–97.2 | 3.0 | 3.0–3.0 |
| $\mathbf{Cu_3SbSe_3}$ | $Pnma$ | 28 | 33 | Yes | 401095 | | Sb | 99.6 | 99.6–99.6 | 3.5 | 3.5–3.5 |
| $\mathbf{Tl_3AsSe_3}$ | $R3m$ | 7 | -33 | Yes | 15148 | Tl3AsSe3 | As | 102.1 | 102.1–102.1 | 3.0 | 3.0–3.0 |
| $Tl_3SbSe_3$ | $P213$ | 28 | -13 | Yes | 60962 | Na3AsS3 | | | | | |

| | | | | | | | | | | | |
|---|---|---|---|---|---|---|---|---|---|---|---|
| **$Ba_2As_2Se_5$** | $P21$ | 36 | -65 | Yes | 60954 | | As | 97.8 | 89.8–101.2 | 3.3 | 3.0–3.6 |
| **$Pb_2Bi_2Se_5$** | $C2/m$ | 9 | 1 | Yes | 30372 | Bi2Pb2Se5 | Bi | 89.9 | 89.9–89.9 | 5.6 | 5.6–5.6 |
| **$Rb_2Bi_4Se_7$** | $P21/m$ | 28 | -59 | Yes | 411071 | | Bi | 89.9 | 89.9–90.0 | 5.7 | 5.2–5.9 |
| **$Cs_2Bi_4Se_7$** | $P21/m$ | 28 | -6 | Yes | 411072 | | Bi | 89.9 | 89.9–90.0 | 5.7 | 5.2–5.9 |
| **$Cs_3Bi_7Se_{12}$** | $Cm$ | 22 | 2 | Yes | 61785 | | Bi | 89.9 | 89.8–90.0 | 5.6 | 5.1–6.0 |
| **$Sr_4Bi_6Se_{13}$** | $P21/m$ | 46 | 1 | Yes | 62782 | K2Bi8Se13 | Bi | 89.2 | 85.1–90.0 | 5.3 | 4.7–5.9 |
| **$Sn_6Bi_2Se_9$** | $Cmcm$ | 34 | 7 | Yes | 422136 | | Bi | 90.0 | 90.0–90.0 | 5.7 | 5.7–5.7 |
| $BaSb_2Se_4$ | $P21/c$ | 56 | -20 | Yes | 32040 | | | | | | |
| **$SrBi_2Se_4$** | $P63/m$ | 86 | 10 | Yes | 51315 | | Bi | 90.0 | 89.9–90.0 | 5.1 | 4.3–5.5 |
| **$EuSb_2Se_4$** | $Pnma$ | 28 | 30 | Yes | 631653 | CaFe2O4 | Sb | 89.9 | 89.8–90.1 | 5.8 | 5.6–6.0 |
| $EuBi_2Se_4$ | $Pnma$ | 28 | 23 | Yes | 616654 | | | | | | |
| $EuBi_2Se_4$ | $Pnma$ | 28 | 26 | Yes | 600805 | | | | | | |
| **$YbSb_2Se_4$** | $Pnma$ | 28 | 68 | Yes | 600795 | CaFe2O4 | Sb | 87.7 | 85.3–90.0 | 5.9 | 5.8–5.9 |
| $MnSb_2Se_4$ | $C2/m$ | 14 | -29 | Yes | 421940 | | | | | | |
| $PbAs_2Se_4$ | $Pnma$ | 28 | 2 | No | | | | | | | |
| $RbSb_3Se_5$ | $P21/c$ | 36 | -13 | Yes | 64672 | RbSb3Se5 | | | | | |
| **$CsBi_3Se_5$** | $Pnma$ | 36 | -11 | Yes | 171610 | Pb2Sb2S5 | Bi | 89.9 | 89.8–90.0 | 5.5 | 5.0–6.0 |
| $CrSbSe_3$ | $Pnma$ | 20 | -11 | Yes | 84866 | NH4CdCl3/Sn2S3 | | | | | |
| **$K_2Bi_8Se_{13}$** | $P\bar{1}$ | 23 | -8 | Yes | 72976 | | Bi | 88.5 | 84.3–90.0 | 5.5 | 4.8–5.9 |
| **$Tl_9SbSe_6$** | $P4/n$ | 32 | -34 | Yes | 56385 | | Sb | 89.8 | 89.8–89.8 | 5.0 | 5.0–5.0 |
| **SbTeI** | $P\bar{1}$ | 6 | -1 | Yes | 35471 | P2I4 | Sb | 89.6 | 89.6–89.6 | 4.7 | 4.7–4.7 |
| **BiTeI** | $P3m1$ | 3 | -26 | Yes | 10500 | | Bi | 92.1 | 92.1–92.1 | 5.7 | 5.7–5.7 |
| **$NaSbTe_2$** | $R\bar{3}m$ | 4 | -30 | No | | | Sb | 90.0 | 90.0–90.0 | 6.0 | 6.0–6.0 |
| **$AgSbTe_2$** | $P4/mmm$ | 4 | 64 | Yes | 170662 | AgSbTe2(tP4) | Sb | 90.0 | 90.0–90.0 | 6.0 | 6.0–6.0 |
| **$AgSbTe_2$** | $R\bar{3}m$ | 4 | 12 | Yes | 170663 | NaCrS2 | Sb | 90.0 | 90.0–90.0 | 6.1 | 6.1–6.1 |
| **$AgBiTe_2$** | $C2/m$ | 12 | 15 | Yes | 604866 | | Bi | 90.0 | 90.0–90.0 | 6.1 | 6.1–6.1 |
| **$AgBiTe_2$** | $C2/m$ | 12 | 94 | Yes | 159345 | AgBiSe2 | Bi | 90.0 | 90.0–90.0 | 5.9 | 5.8–6.0 |
| **$AgBiTe_2$** | $R\bar{3}m$ | 4 | 16 | Yes | 43266 | NaCrS2 | Bi | 90.0 | 90.0–90.0 | 6.1 | 6.1–6.1 |
| **$TlSbTe_2$** | $R\bar{3}m$ | 4 | -35 | Yes | 15411 | NaCrS2 | Sb | 90.0 | 90.0–90.0 | 6.0 | 6.0–6.0 |
| **$TlBiTe_2$** | $R\bar{3}m$ | 4 | -65 | Yes | 15412 | NaCrS2 | Bi | 90.0 | 90.0–90.0 | 6.0 | 6.0–6.0 |
| **$Na_3SbTe_3$** | $P213$ | 28 | 25 | Yes | 75513 | Na3AsS3 | Sb | 98.9 | 98.9–98.9 | 3.2 | 3.2–3.2 |
| **$K_3SbTe_3$** | $P213$ | 28 | -66 | Yes | 71301 | Na3AsS3 | Sb | 102.8 | 102.8–102.8 | 3.0 | 3.0–3.0 |
| **$K_3BiTe_3$** | $P213$ | 28 | -51 | Yes | 300183 | Na3AsS3 | Bi | 101.3 | 101.3–101.3 | 3.0 | 3.0–3.0 |
| **$Ge_3As_2Te_6$** | $R\bar{3}m$ | 11 | 14 | Yes | 68113 | As2Ge3Te6 | As | 90.0 | 90.0–90.0 | 5.8 | 5.8–5.8 |
| **$Ge_3Sb_2Te_6$** | $R\bar{3}m$ | 11 | 9 | Yes | 157728 | | Sb | 90.0 | 90.0–90.0 | 5.8 | 5.8–5.8 |
| **$Ge_3Bi_2Te_6$** | $R3m$ | 11 | 32 | Yes | 16207 | | Bi | 90.0 | 90.0–90.0 | 5.9 | 5.8–5.9 |
| **$Ge_2As_2Te_5$** | $P\bar{3}m1$ | 9 | 13 | Yes | 68112 | Bi2Pb2Se5 | As | 90.0 | 90.0–90.0 | 5.8 | 5.8–5.8 |
| **$Ge_2Sb_2Te_5$** | $C2/m$ | 9 | 5 | Yes | 55295 | | Sb | 90.0 | 90.0–90.0 | 5.8 | 5.8–5.8 |
| **$Ge_2Sb_2Te_5$** | $P\bar{3}m1$ | 9 | 20 | Yes | 42876 | Bi2Pb2Se5 | Sb | 90.0 | 90.0–90.0 | 5.9 | 5.9–5.9 |
| **$Ge_2Bi_2Te_5$** | $P\bar{3}m1$ | 9 | 11 | Yes | 249302 | | Bi | 90.0 | 90.0–90.0 | 5.8 | 5.8–5.8 |
| **$Pb_2Bi_2Te_5$** | $P\bar{3}m1$ | 9 | 59 | Yes | 42708 | Bi2Pb2Se5 | Bi | 90.0 | 90.0–90.0 | 5.8 | 5.8–5.8 |
| **$Ge_4As_2Te_7$** | $R\bar{3}m$ | 13 | 14 | Yes | 68114 | | As | 89.9 | 89.9–89.9 | 5.8 | 5.8–5.8 |
| **$Ge_5As_2Te_8$** | $P\bar{3}m1$ | 15 | 15 | Yes | 63174 | | As | 89.9 | 89.9–89.9 | 5.8 | 5.8–5.8 |
| **$GeAs_2Te_4$** | $R\bar{3}m$ | 7 | 12 | Yes | 68111 | In3Te4(HP) | As | 90.0 | 90.0–90.0 | 5.8 | 5.8–5.8 |
| **$GeBi_2Te_4$** | $R\bar{3}m$ | 7 | 6 | Yes | 30394 | In3Te4(HP) | Bi | 90.0 | 90.0–90.0 | 5.8 | 5.8–5.8 |
| **$PbBi_2Te_4$** | $R\bar{3}m$ | 7 | 3 | Yes | 616936 | GeSb2Te4 | Bi | 90.0 | 90.0–90.0 | 5.8 | 5.8–5.8 |
| **$SnSb_2Te_4$** | $R\bar{3}m$ | 7 | 1 | Yes | 30392 | In3Te4(HP) | Sb | 90.0 | 90.0–90.0 | 5.8 | 5.8–5.8 |
| **$PbSb_2Te_4$** | $R\bar{3}m$ | 7 | 8 | Yes | 250250 | | Sb | 90.0 | 90.0–90.0 | 5.8 | 5.8–5.8 |
| **$GeAs_4Te_7$** | $P\bar{3}m1$ | 12 | 10 | Yes | 41107 | AgBiSe2 | As | 90.0 | 90.0–90.0 | 5.8 | 5.8–5.9 |
| **$GeSb_4Te_7$** | $P\bar{3}m1$ | 12 | 0 | Yes | 42875 | AgBiSe2 | Sb | 90.0 | 90.0–90.0 | 5.8 | 5.8–5.9 |
| **$GeBi_4Te_7$** | $C2/m$ | 12 | 2 | Yes | 42891 | AgBiSe2 | Bi | 90.0 | 89.9–90.0 | 5.8 | 5.7–5.8 |
| **$PbBi_4Te_7$** | $C2/m$ | 12 | 1 | Yes | 42753 | AgBiSe2 | Bi | 90.0 | 90.0–90.0 | 5.8 | 5.8–5.8 |
| **$Tl_9SbTe_6$** | $I4/m$ | 16 | -20 | Yes | 55583 | | Sb | 90.0 | 90.0–90.0 | 6.8 | 6.8–6.8 |
| **$PbBi_6Te_{10}$** | $R\bar{3}m$ | 17 | 1 | Yes | 95551 | Bi8Se9 | Bi | 90.0 | 90.0–90.0 | 5.8 | 5.8–5.8 |
| $CeBiS_2O$ | $P4/nmm$ | 10 | 15 | Yes | 80 | | | | | | |
| **$LaBiSe_2O$** | $P4/nmm$ | 10 | 8 | No | | | Bi | 89.5 | 89.5–89.5 | 4.6 | 4.6–4.6 |

| | | | | | | | | | | | |
|---|---|---|---|---|---|---|---|---|---|---|---|
| $Ag_2Bi_2S_3Cl_2$ | $P\bar{1}$ | 36 | -4 | Yes | 412076 | | | | | | |
| $MnSbS_2Cl$ | $Pnma$ | 20 | -6 | Yes | 151925 | | | | | | |
| $\mathbf{MnBiS_2Cl}$ | $Pnma$ | 20 | -18 | Yes | 172156 | | Bi | 85.1 | 85.1–85.1 | 4.5 | 4.5–4.5 |
| $CdSbS_2Cl$ | $Pnma$ | 20 | 4 | Yes | 171722 | | | | | | |
| $\mathbf{CdBiS_2Cl}$ | $Pnma$ | 20 | 10 | Yes | 171724 | | Bi | 85.4 | 85.4–85.4 | 4.6 | 4.6–4.6 |
| $\mathbf{AgBi_2S_3Cl}$ | $P21/m$ | 14 | 7 | Yes | 412372 | | Bi | 86.1 | 85.9–86.3 | 5.4 | 5.1–5.7 |
| $Hg_3AsS_4Cl$ | $P63mc$ | 18 | 4 | Yes | 280329 | Hg3SAsS3Cl | | | | | |
| $InSb_2S_4Cl$ | $C2/m$ | 16 | -16 | Yes | 159468 | InSb2S4Cl | | | | | |
| $\mathbf{InBi_2S_4Cl}$ | $C2/m$ | 8 | -2 | Yes | 484 | | Bi | 87.0 | 87.0–87.0 | 5.4 | 5.4–5.4 |
| $\mathbf{AlBiSCl_4}$ | $I\bar{4}$ | 28 | -26 | Yes | 414154 | Bi4Te4(AlCl4)4 | Bi | 87.4 | 87.4–87.4 | 5.0 | 5.0–5.0 |
| $LaSbS_2Br_2$ | $P21/c$ | 48 | -15 | Yes | 93666 | | | | | | |
| $CeSbS_2Br_2$ | $P21/c$ | 48 | -16 | Yes | 93664 | | | | | | |
| $MnSbS_2Br$ | $C2/m$ | 10 | -7 | Yes | 172782 | CdSbS2Br | | | | | |
| $MnBiS_2Br$ | $C2/m$ | 10 | -13 | Yes | 415307 | AgBi3S4Br2 | | | | | |
| $CdSbS_2Br$ | $C2/m$ | 10 | 13 | Yes | 171723 | CdSbS2Br | | | | | |
| $CdBiS_2Br$ | $C2/m$ | 10 | 16 | Yes | 171725 | CdSbS2Br | | | | | |
| $Hg_3AsS_4Br$ | $P63mc$ | 18 | 2 | Yes | 280330 | Hg3SAsS3Cl | | | | | |
| $InSb_2S_4Br$ | $C2/m$ | 16 | -3 | Yes | 159467 | InSb2S4Cl | | | | | |
| $Ce_2SbS_5Br$ | $Pnma$ | 36 | 3 | Yes | 51484 | | | | | | |
| $Pb_2SbS_2I_3$ | $P21/c$ | 32 | 20 | Yes | 418344 | | | | | | |
| $CdSb_6S_8I_4$ | $P\bar{1}$ | 19 | 1 | Yes | 27733 | | | | | | |
| $\mathbf{Ag_3Tl_3As_2S_6}$ | $P21/c$ | 56 | -16 | Yes | 160101 | Tl3Ag3(AsS3)2 | As | 101.2 | 100.7–101.8 | 3.0 | 3.0–3.0 |
| $Ag_3Tl_3Sb_2S_6$ | $P21/c$ | 56 | -9 | Yes | 160100 | Tl3Ag3(AsS3)2 | | | | | |
| $\mathbf{KCu_2AsS_3}$ | $P\bar{1}$ | 28 | -11 | Yes | 75429 | | As | 103.2 | 103.0–103.3 | 3.7 | 3.6–3.8 |
| $\mathbf{K_2CuSbS_3}$ | $P21/c$ | 28 | -0 | Yes | 415483 | | Sb | 100.4 | 100.4–100.4 | 3.4 | 3.4–3.4 |
| $\mathbf{KAg_2SbS_3}$ | $P\bar{1}$ | 28 | -1 | Yes | 420015 | | Sb | 100.8 | 100.0–101.5 | 3.2 | 3.2–3.3 |
| $\mathbf{CsAg_2AsS_3}$ | $P21/c$ | 28 | -46 | Yes | 421091 | | As | 101.3 | 101.3–101.3 | 3.1 | 3.1–3.1 |
| $\mathbf{CsAg_2BiS_3}$ | $P21/c$ | 28 | -15 | Yes | 93372 | | Bi | 90.0 | 90.0–90.0 | 5.8 | 5.8–5.8 |
| $Na_2CuSbS_3$ | $P21/c$ | 28 | -8 | Yes | 81678 | | | | | | |
| $K_2Ag_3Sb_3S_7$ | $Cmc21$ | 32 | 11 | Yes | 420016 | | | | | | |
| $\mathbf{Cu_6Hg_3As_4S_{12}}$ | $R3$ | 25 | 2 | Yes | 20424 | Cu6Zn3(AsS3)4 | As | 100.5 | 99.0–101.0 | 3.0 | 3.0–3.0 |
| $LiEuAsS_3$ | $P21/c$ | 24 | -1 | Yes | 249705 | ZnP2(mP) | | | | | |
| $\mathbf{KEuAsS_3}$ | $P21/c$ | 24 | -17 | Yes | 249706 | KEuAsS3 | As | 100.4 | 100.4–100.4 | 3.0 | 3.0–3.0 |
| $\mathbf{RbEuAsS_3}$ | $P21/c$ | 24 | -89 | Yes | 249707 | KEuAsS3 | As | 100.8 | 100.8–100.8 | 3.0 | 3.0–3.0 |
| $EuCuSbS_3$ | $Pmn21$ | 24 | -10 | No | | | | | | | |
| $\mathbf{CuPbAsS_3}$ | $Pmn21$ | 24 | -4 | Yes | 14304 | CuPbAsS3 | As | 97.6 | 97.6–97.7 | 3.0 | 3.0–3.0 |
| $AgPbAsS_3$ | $P21/c$ | 24 | -1 | Yes | 26835 | Ag2SeO3 | | | | | |
| $CuPbSbS_3$ | $Pmn21$ | 24 | 2 | Yes | 182267 | | | | | | |
| $CuPbSbS_3$ | $Pmn21$ | 24 | 1 | Yes | 14303 | CuPbAsS3 | | | | | |
| $AgPbSbS_3$ | $P21/c$ | 24 | 46 | Yes | 24257 | Ag2SeO3 | | | | | |
| $AgPbSbS_3$ | $P21/c$ | 24 | 15 | Yes | 8166 | Ag2SeO3 | | | | | |
| $\mathbf{CsEuAsS_3}$ | $P21/c$ | 24 | -89 | Yes | 249708 | KEuAsS3 | As | 101.1 | 101.1–101.1 | 3.0 | 3.0–3.0 |
| $KHgSbS_3$ | $C2/c$ | 24 | 14 | Yes | 63623 | | | | | | |
| $KHgSbS_3$ | $C2/c$ | 24 | 14 | Yes | 655286 | | | | | | |
| $\mathbf{AgHgAsS_3}$ | $Cc$ | 12 | -1 | Yes | 31194 | | As | 97.7 | 97.7–97.7 | 3.0 | 3.0–3.0 |
| $\mathbf{HgTlAsS_3}$ | $P21/c$ | 24 | 4 | Yes | 33705 | | As | 101.8 | 101.8–101.8 | 3.0 | 3.0–3.0 |
| $CuPbBiS_3$ | $Pnma$ | 24 | 9 | Yes | 9120 | Eu2CuS3 | | | | | |
| $Cs_3Ag_2Sb_3S_8$ | $P21/m$ | 32 | -5 | Yes | 55365 | | | | | | |
| $MnAg_4Sb_2S_6$ | $P21/c$ | 26 | 24 | Yes | 26141 | Ag4MnSb2S6 | | | | | |
| $\mathbf{Cs_2ZnBi_2S_5}$ | $Pnma$ | 40 | -33 | Yes | 97426 | Cs2Bi2ZnS5 | Bi | 90.0 | 90.0–90.1 | 5.7 | 5.2–6.2 |
| $\mathbf{Cs_2CdBi_2S_5}$ | $Pnma$ | 40 | -33 | Yes | 97427 | Cs2Bi2ZnS5 | Bi | 90.0 | 90.0–90.0 | 5.3 | 4.7–5.9 |
| $\mathbf{MnTl_2As_2S_5}$ | $Cmca$ | 40 | 13 | Yes | 17035 | | As | 97.8 | 97.8–97.8 | 3.0 | 3.0–3.0 |
| $\mathbf{KCu_4AsS_4}$ | $P21$ | 20 | -1 | Yes | 75430 | | As | 99.2 | 99.2–99.2 | 3.0 | 3.0–3.0 |
| $\mathbf{KAg_2AsS_4}$ | $I\bar{4}2m$ | 8 | -19 | No | | | As | 109.2 | 109.2–109.2 | 4.0 | 4.0–4.0 |
| $\mathbf{K_2AuAsS_4}$ | $P21/m$ | 16 | -23 | Yes | 85681 | K2AuOS4 | As | 103.1 | 103.1–103.1 | 4.0 | 4.0–4.0 |
| $\mathbf{KCuBi_2S_4}$ | $Cmc21$ | 16 | 1 | Yes | 91297 | KBi2CuS4 | Bi | 90.0 | 90.0–90.0 | 6.1 | 5.8–6.3 |

| | | | | | | | | | | | |
|---|---|---|---|---|---|---|---|---|---|---|---|
| **$KAg_2SbS_4$** | $I\bar{4}2m$ | 8 | 0 | Yes | 82143 | K3VO4 | Sb | 109.5 | 109.5–109.5 | 4.0 | 4.0–4.0 |
| **$RbAg_2SbS_4$** | $I\bar{4}2m$ | 8 | 11 | No | | | Sb | 107.8 | 107.8–107.8 | 4.0 | 4.0–4.0 |
| **$RbAg_2SbS_4$** | $P3221$ | 24 | -3 | Yes | 82145 | Cu2SnSrS4 | Sb | 109.0 | 109.0–109.0 | 4.0 | 4.0–4.0 |
| **$Rb_2AuSbS_4$** | $Pbcm$ | 32 | -5 | Yes | 54507 | | Sb | 103.7 | 103.7–103.7 | 4.0 | 4.0–4.0 |
| **$CsCuBi_2S_4$** | $Cmc21$ | 16 | 22 | Yes | 93370 | KBi2CuS4 | Bi | 90.1 | 90.0–90.2 | 5.4 | 5.2–5.6 |
| **$Ag_2TlSbS_4$** | $I\bar{4}2m$ | 8 | 15 | No | | | Sb | 109.3 | 109.3–109.3 | 4.0 | 4.0–4.0 |
| **$K_3Cu_2Bi_5S_{10}$** | $Pnnm$ | 40 | -17 | Yes | 93369 | ScU3S6 | Bi | 90.0 | 89.9–90.0 | 6.0 | 5.7–6.3 |
| **$Rb_3Cu_2Bi_5S_{10}$** | $Pnnm$ | 40 | -16 | Yes | 91298 | ScU3S6 | Bi | 90.0 | 89.9–90.1 | 5.8 | 5.3–6.2 |
| **$Cs_3Cu_2Bi_5S_{10}$** | $Pnnm$ | 40 | 7 | Yes | 91299 | ScU3S6 | Bi | 90.0 | 89.9–90.1 | 5.5 | 4.7–6.0 |
| **$Ag_3BiSb_2S_6$** | $P\bar{1}$ | 24 | 9 | Yes | 94646 | | Bi | 90.2 | 90.2–90.2 | 5.4 | 5.4–5.4 |
| **$Cs_4Cu_3Bi_9S_{17}$** | $P21/m$ | 66 | 10 | No | | | Bi | 90.0 | 89.7–90.1 | 5.8 | 5.2–6.6 |
| $K_2SnAs_2S_6$ | $P\bar{3}$ | 11 | -31 | Yes | 281039 | Tl2Sn(AsS3)2 | | | | | |
| **$Tl_2SnAs_2S_6$** | $P\bar{3}$ | 11 | -10 | Yes | 72907 | Tl2Sn(AsS3)2 | As | 97.1 | 97.1–97.1 | 3.0 | 3.0–3.0 |
| **$Cu_2Pb_6Bi_8S_{19}$** | $C2/m$ | 35 | 2 | Yes | 411110 | | Bi | 87.6 | 80.6–90.0 | 5.0 | 4.2–6.0 |
| $Ba_2FeSbS_5$ | $Pnma$ | 36 | -14 | Yes | 261418 | | | | | | |
| $Ba_2FeBiS_5$ | $Pnma$ | 36 | 10 | Yes | 261419 | | | | | | |
| $Ba_2GaBiS_5$ | $Pnma$ | 36 | -24 | Yes | 261677 | | | | | | |
| **$Ba_2InBiS_5$** | $Cmc21$ | 18 | -62 | Yes | 261678 | | Bi | 89.8 | 89.8–89.8 | 4.9 | 4.9–4.9 |
| $BaBSbS_4$ | $Pnma$ | 28 | -46 | Yes | 248221 | | | | | | |
| $KSiBiS_4$ | $P21/c$ | 28 | -120 | Yes | 421485 | Pb2SiS4 | | | | | |
| $BaBBiS_4$ | $C2/m$ | 14 | -22 | Yes | 248222 | | | | | | |
| $RbSiBiS_4$ | $P21/c$ | 28 | -51 | Yes | 281166 | Pb2SiS4 | | | | | |
| $KGeBiS_4$ | $P21/c$ | 28 | -13 | Yes | 421486 | Pb2SiS4 | | | | | |
| $CsSiBiS_4$ | $P21/c$ | 28 | -57 | Yes | 281169 | | | | | | |
| $RbGeBiS_4$ | $P21/c$ | 28 | -14 | Yes | 281167 | Pb2SiS4 | | | | | |
| $CsGeBiS_4$ | $P21/c$ | 28 | -16 | Yes | 281168 | Pb2SiS4 | | | | | |
| $FeBiSbS_4$ | $Pnma$ | 28 | 173 | Yes | 155236 | CaFe2O4 | | | | | |
| $YbCuBi_3S_6$ | $Pmc21$ | 22 | 13 | No | | | | | | | |
| $CuPbBi_3S_6$ | $Pmc21$ | 22 | 5 | Yes | 95926 | Bi3CuPbS6 | | | | | |
| $Nd_2Mn_3Sb_4S_{12}$ | $C2/m$ | 21 | 9 | Yes | 422013 | | | | | | |
| $Sm_2Mn_3Sb_4S_{12}$ | $C2/m$ | 21 | 12 | Yes | 422014 | | | | | | |
| $Pr_2Mn_3Sb_4S_{12}$ | $C2/m$ | 21 | 9 | Yes | 422012 | | | | | | |
| $Gd_2Mn_3Sb_4S_{12}$ | $C2/m$ | 21 | 16 | Yes | 422015 | | | | | | |
| **$K_9BiP_4S_{16}$** | $P21212$ | 60 | -104 | Yes | 173368 | | Bi | 85.9 | 85.9–85.9 | 6.3 | 6.3–6.3 |
| $K_3BiP_2S_8$ | $P212121$ | 56 | -28 | Yes | 81772 | | | | | | |
| $MnPb_4Sb_6S_{14}$ | $P21/c$ | 50 | 1 | Yes | 98581 | | | | | | |
| $FePb_4Sb_6S_{14}$ | $P21/c$ | 50 | 41 | Yes | 24256 | | | | | | |
| **$LiSn_2Bi_5S_{10}$** | $P2/m$ | 36 | 0 | No | | | Bi | 86.1 | 80.3–90.0 | 5.1 | 4.7–5.6 |
| $NaSn_2Bi_5S_{10}$ | $P2/m$ | 36 | 10 | No | | | | | | | |
| **$BeLa_3SbS_7$** | $P63$ | 24 | 90 | Yes | 616308 | | Sb | 89.6 | 89.6–89.6 | 5.1 | 5.1–5.1 |
| **$BeLa_3BiS_7$** | $P63$ | 24 | 111 | Yes | 616183 | | Bi | 89.9 | 89.9–89.9 | 6.8 | 6.8–6.8 |
| $In_2GaBiS_6$ | $P21/m$ | 20 | 0 | Yes | 410032 | Bi2Ga2In4S12 | | | | | |
| $Pr_4GaSbS_9$ | $Aba2$ | 60 | -14 | Yes | 261382 | | | | | | |
| $Sm_4GaSbS_9$ | $Aba2$ | 60 | -14 | Yes | 261384 | | | | | | |
| $Gd_4GaSbS_9$ | $Aba2$ | 60 | -10 | Yes | 261385 | | | | | | |
| $SrSbSe_2F$ | $P4/nmm$ | 10 | 8 | Yes | 171430 | | | | | | |
| $BaSbSe_2F$ | $P\bar{1}$ | 20 | -15 | Yes | 171429 | | | | | | |
| **$AgBi_2Se_3Cl$** | $P21/m$ | 14 | -1 | Yes | 412371 | | Bi | 87.2 | 86.6–87.9 | 5.7 | 5.2–6.1 |
| **$AlBiSeCl_4$** | $I\bar{4}$ | 28 | -28 | Yes | 414155 | Bi4Te4(AlCl4)4 | Bi | 89.3 | 89.3–89.3 | 5.5 | 5.5–5.5 |
| $MnSbSe_2Br$ | $Pnma$ | 20 | 6 | Yes | 172784 | | | | | | |
| $MnBiSe_2Br$ | $Pnma$ | 24 | -4 | Yes | 172783 | | | | | | |
| **$CdBiSe_2Br$** | $Pnma$ | 20 | 21 | Yes | 171726 | | Bi | 86.4 | 86.4–86.4 | 4.6 | 4.6–4.6 |
| $CdSb_2Se_3Br_2$ | $C2/m$ | 16 | -6 | Yes | 159464 | InSb2S4Cl | | | | | |
| $Hg_3AsSe_4Br$ | $P63mc$ | 18 | -3 | Yes | 280331 | Hg3SAsS3Cl | | | | | |
| $InSb_2Se_4Br$ | $C2/m$ | 16 | -8 | Yes | 159466 | InSb2S4Cl | | | | | |
| $InBi_2Se_4Br$ | $C2/m$ | 16 | 5 | Yes | 159465 | InSb2S4Cl | | | | | |

| | | | | | | | | | | | |
|---|---|---|---|---|---|---|---|---|---|---|---|
| $MnSbSe_2I$ | $C2/m$ | 10 | 3 | Yes | 281558 | CdSbS2Br | | | | | |
| $MnBiSe_2I$ | $C2/m$ | 10 | -5 | Yes | 415138 | AgBi3S4Br2 | | | | | |
| $CdBiSe_2I$ | $C2/m$ | 10 | 37 | Yes | 171727 | CdSbS2Br | | | | | |
| $Hg_3AsSe_4I$ | $P63mc$ | 18 | -3 | Yes | 280332 | Hg3SAsS3Cl | | | | | |
| $In_2BiSe_4I$ | $Pnma$ | 32 | 8 | Yes | 423015 | | | | | | |
| $Cs_2Cu_2Sb_2Se_5$ | $P\bar{1}$ | 22 | -7 | Yes | 88681 | | | | | | |
| **$RbK_2BiSe_3$** | $P213$ | 28 | -11 | Yes | 85412 | Na3AsS3 | Bi | 101.2 | 101.2–101.2 | 3.0 | 3.0–3.0 |
| $RbHgSbSe_3$ | $P21/c$ | 24 | -15 | Yes | 89018 | | | | | | |
| **$Rb_2ZnBi_2Se_5$** | $Pnma$ | 40 | -38 | No | | | Bi | 90.0 | 90.0–90.0 | 5.8 | 5.4–6.3 |
| **$Cs_2ZnBi_2Se_5$** | $Pnma$ | 40 | -37 | Yes | 59855 | Cs2Bi2ZnS5 | Bi | 90.0 | 90.0–90.0 | 5.8 | 5.3–6.2 |
| **$KAg_2SbSe_4$** | $I\bar{4}2m$ | 8 | 14 | No | | | Sb | 109.3 | 109.3–109.3 | 4.0 | 4.0–4.0 |
| **$RbAg_2As_3Se_6$** | $P\bar{1}$ | 48 | -12 | Yes | 88005 | | As | 97.2 | 91.7–101.0 | 3.0 | 3.0–3.0 |
| **$Rb_2AgAs_3Se_6$** | $P21/c$ | 48 | -12 | Yes | 88004 | K2AgAs3Se6 | As | 98.6 | 95.8–102.0 | 3.0 | 2.9–3.0 |
| $Cs_3GeAsSe_5$ | $P21/c$ | 40 | -4 | Yes | 415214 | | | | | | |
| **$Ag_2PbBi_4Se_8$** | $P21/m$ | 36 | 12 | Yes | 181126 | | Bi | 86.7 | 77.0–90.0 | 5.2 | 4.7–5.8 |
| **$K_3BiAs_6Se_{12}$** | $P\bar{3}$ | 22 | -20 | Yes | 180763 | | As | 100.1 | 100.1–100.1 | 3.0 | 3.0–3.0 |
| **$K_3BiAs_6Se_{12}$** | $P\bar{3}$ | 22 | -20 | Yes | 180763 | | Bi | 90.0 | 90.0–90.0 | 6.2 | 6.2–6.2 |
| **$KSm_2Sb_3Se_8$** | $Pnma$ | 56 | -19 | Yes | 54799 | | Sb | 90.0 | 90.0–90.0 | 4.8 | 4.5–5.4 |
| **$InSn_2Bi_3Se_8$** | $C2/m$ | 14 | 9 | Yes | 420150 | | Bi | 89.9 | 89.9–90.0 | 5.7 | 5.6–6.0 |
| **$Ag_2CdBi_6Se_{11}$** | $C2/m$ | 20 | 24 | No | | | Bi | 86.8 | 80.5–90.0 | 5.6 | 4.7–6.0 |
| **$CdSnBi_4Se_8$** | $C2/m$ | 14 | 16 | No | | | Bi | 85.2 | 80.6–89.9 | 5.2 | 4.7–5.7 |
| $CdPbBi_4Se_8$ | $Cm$ | 14 | 16 | No | | | | | | | |
| **$AlBiTeCl_4$** | $I\bar{4}$ | 28 | -16 | Yes | 411714 | Bi4Te4(AlCl4)4 | Bi | 90.7 | 90.7–90.7 | 6.2 | 6.2–6.2 |
| **$CsPbBiTe_3$** | $Cmcm$ | 12 | 9 | No | | | Bi | 109.0 | 109.0–109.0 | 4.0 | 4.0–4.0 |
| **$KHgBiTe_3$** | $Cmcm$ | 12 | -16 | No | | | Bi | 90.0 | 90.0–90.0 | 7.3 | 7.3–7.3 |
| **$RbHgBiTe_3$** | $Cmcm$ | 12 | -27 | No | | | Bi | 90.0 | 90.0–90.0 | 7.2 | 7.2–7.2 |
| **$CsHgBiTe_3$** | $Cmcm$ | 12 | -58 | No | | | Bi | 90.0 | 90.0–90.0 | 7.0 | 7.0–7.0 |
| **$Cs_6Cd_2Bi_8Te_{17}$** | $P2/m$ | 66 | -73 | No | | | Bi | 90.0 | 89.8–90.0 | 5.9 | 5.5–6.3 |
| **$H_6C_3BiN_3S_6$** | $P\bar{1}$ | 38 | 57 | Yes | 422349 | | Bi | 80.6 | 80.6–80.6 | 8.5 | 8.5–8.5 |
| $Pb_4As_2S_6ICl$ | $Pmn21$ | 28 | 3 | Yes | 245805 | | | | | | |
| $Cs_2CeAsS_3Cl_2$ | $Pnma$ | 36 | -1 | Yes | 246010 | | | | | | |
| **$AgCu_2PbBiS_4$** | $Pnma$ | 40 | 14 | Yes | 167006 | | Bi | 90.0 | 90.0–90.0 | 5.6 | 5.6–5.6 |
| **$AlSb_2Te_2BrCl_4$** | $C2/c$ | 40 | -21 | Yes | 174524 | | Sb | 88.9 | 88.8–89.0 | 5.7 | 5.7–5.8 |
| **$Cs_2NaC_6BiN_6S_6$** | $P\bar{3}$ | 22 | 110 | Yes | 79593 | | Bi | 90.0 | 90.0–90.0 | 7.1 | 7.1–7.1 |

# References


[S1] Atabaeva, E. Y.; Itskevich, E.; Mashkov, S.; Popova, S.; Vereschagin, L. Bismuth Telluride Polymorphism Under High Pressures and Temperatures. *Sov. Phys. Solid. State* **1968**, 43.

[S2] Pinsker, G.; Semiletov, S.; Belova, E. Electron Diffraction Study of the Structure of $Tl_2Sb_2Se_4$. *Doklady Akademii Nauk SSSR* **1956**, *106*, 1003–1006.

[S3] Wacker, K.; Buck, P. X-ray investigations of thallium-antimony selenide $TlSbSe_2$. *Mater. Res. Bull.* **1980**, *15*, 1105–1111.

[S4] Isaacs, E. B.; Wolverton, C. Inverse Band Structure Design via Materials Database Screening: Application to Square Planar Thermoelectrics. *Chem. Mater.* **2018**, *30*, 1540–1546.

[S5] Topa, D.; Makovicky, E.; Putz, H. The Crystal Structure of Angelaite, $Cu_2AgPbBiS_4$. *Can. Mineral.* **2010**, *48*, 145–153.

[S6] Kirklin, S.; Saal, J. E.; Meredig, B.; Thompson, A.; Doak, J. W.; Aykol, M.; Rühl, S.; Wolverton, C. The Open Quantum Materials Database (OQMD): assessing the accuracy of DFT formation energies. *npj Comput. Mater.* **2015**, *1*, 15010.

[S7] Medeiros, P. V. C.; Stafström, S.; Björk, J. Effects of extrinsic and intrinsic perturbations on the electronic structure of graphene: Retaining an effective primitive cell band structure by band unfolding. *Phys. Rev. B* **2014**, *89*, 041407.
